# Supplementary material for: Memory in quantum dot blinking
Source: arXiv:2106.12179 ancillary file (2021-06-24)

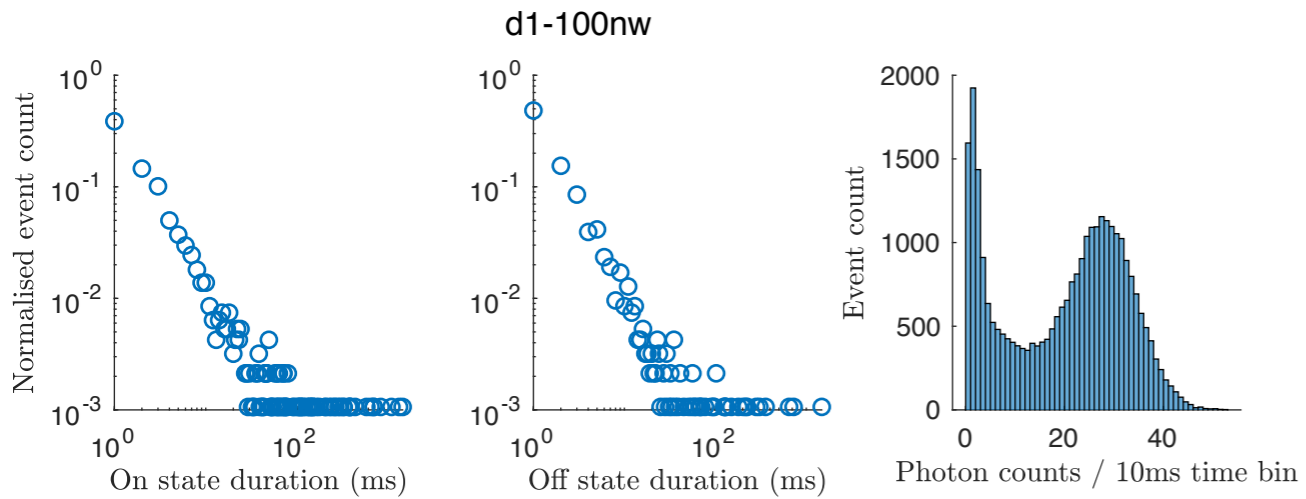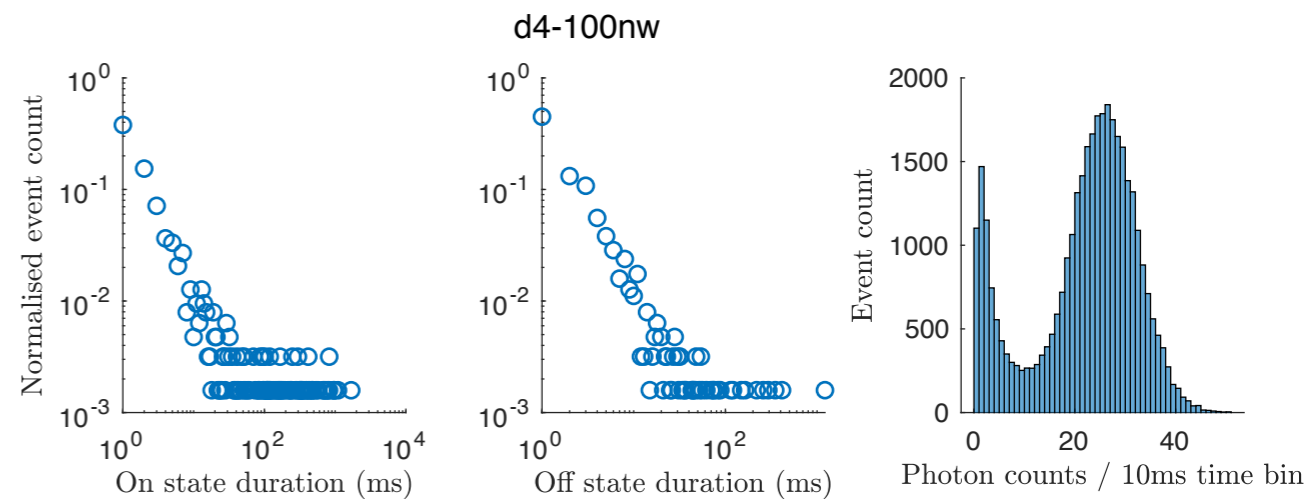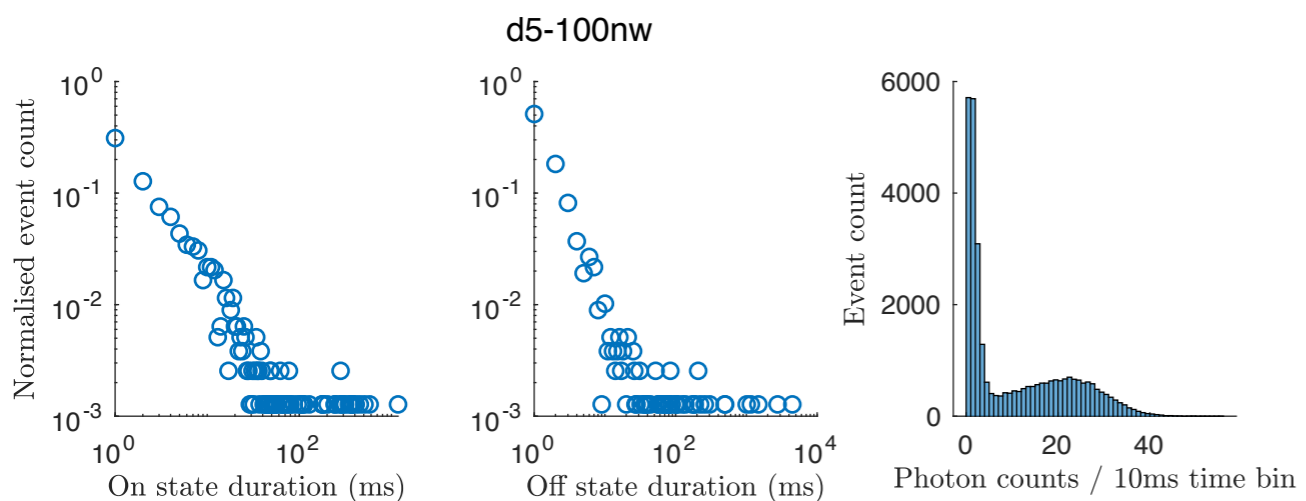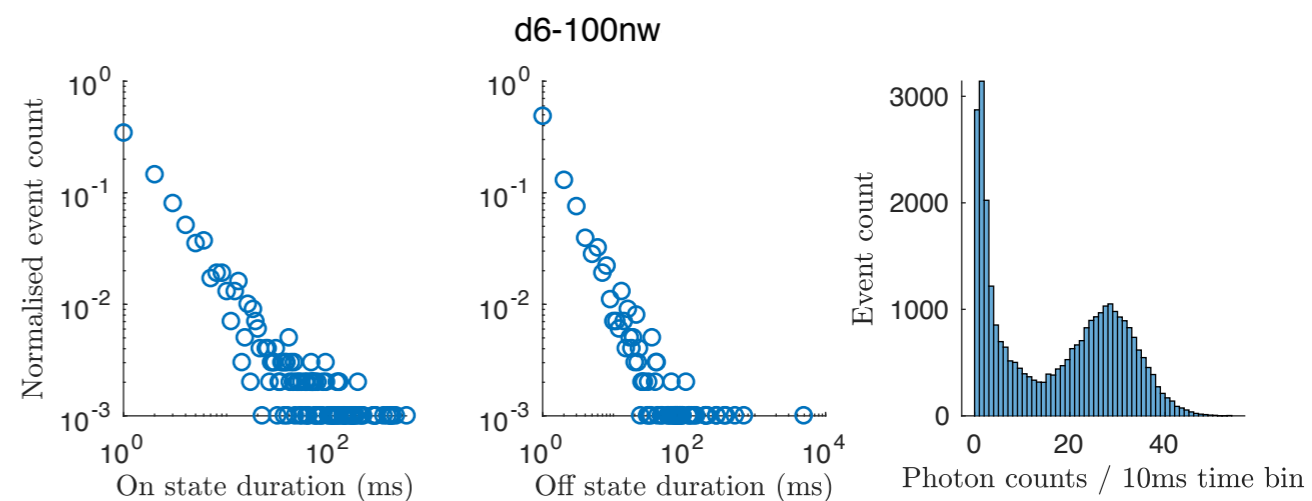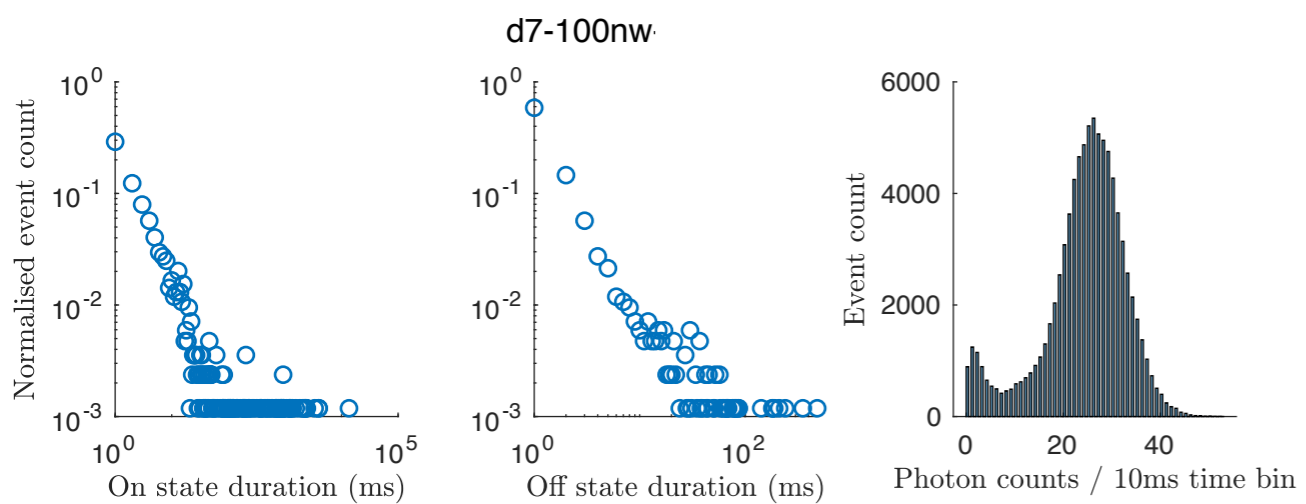

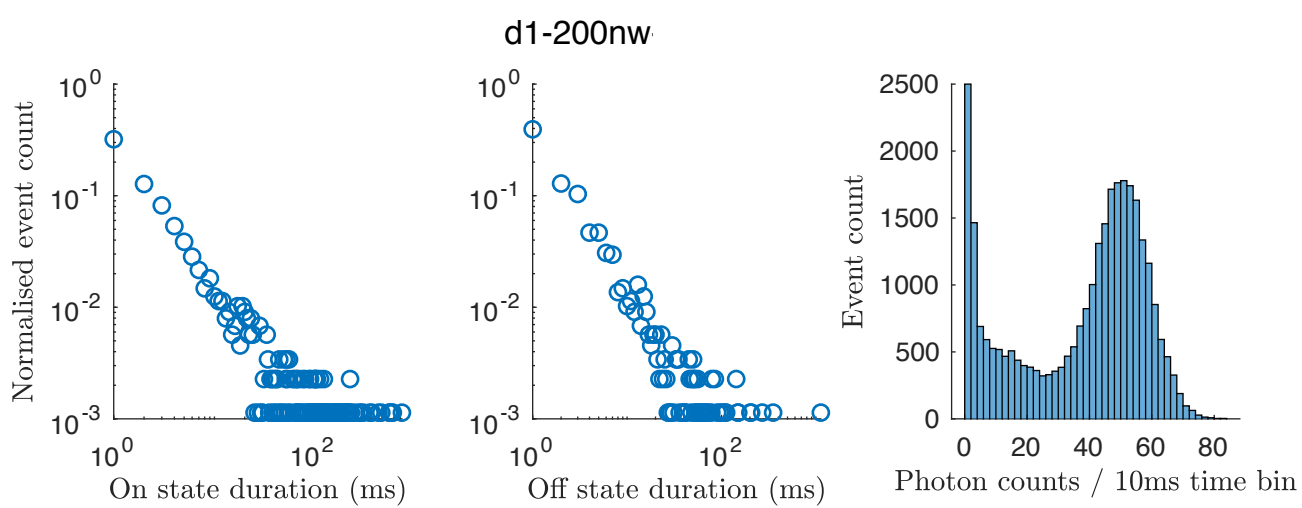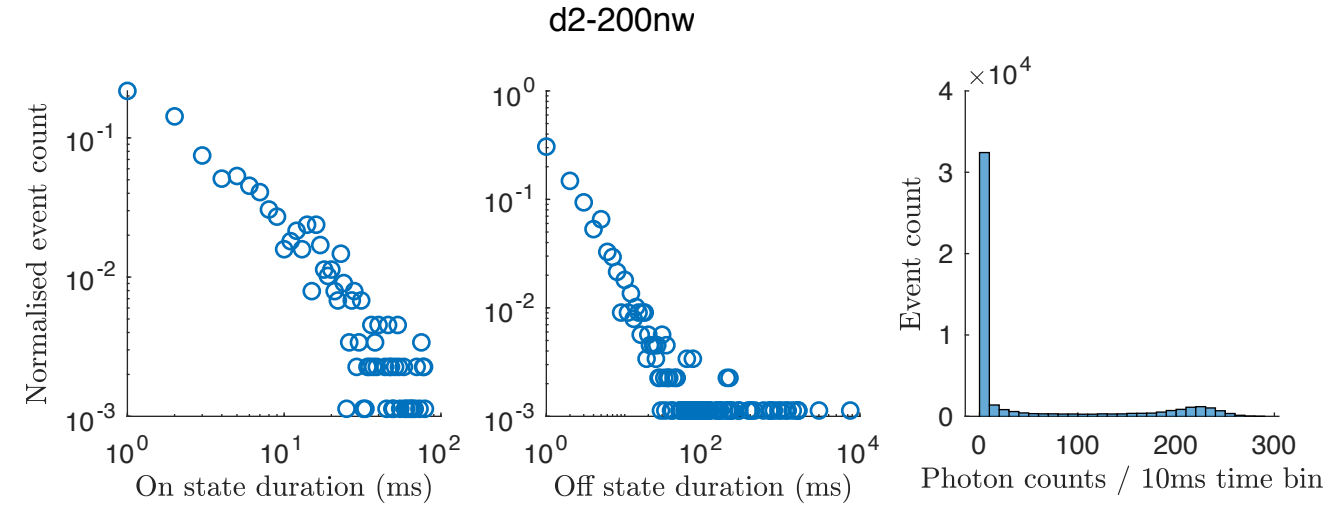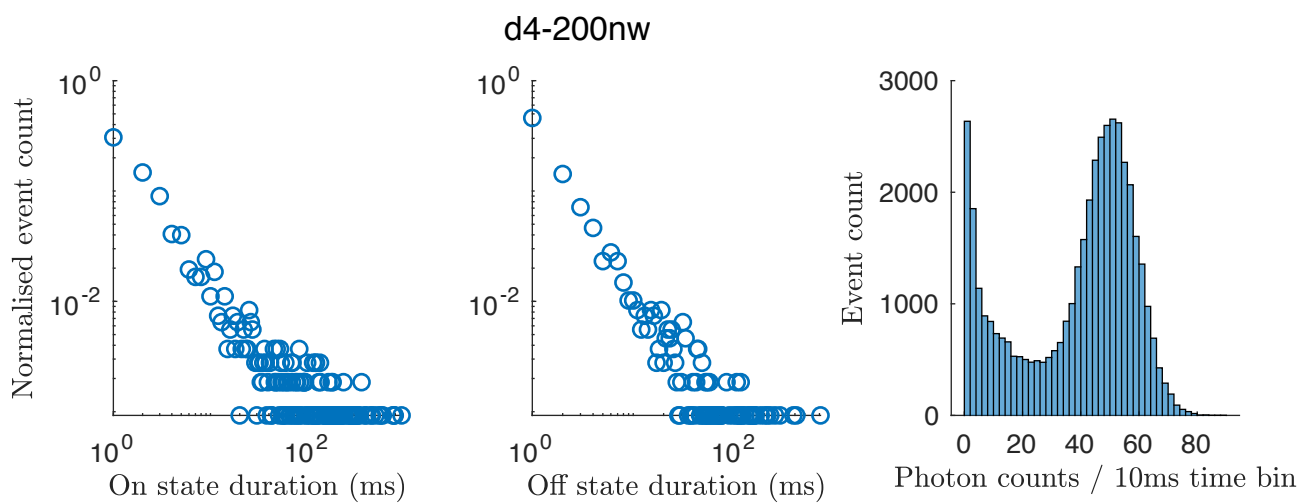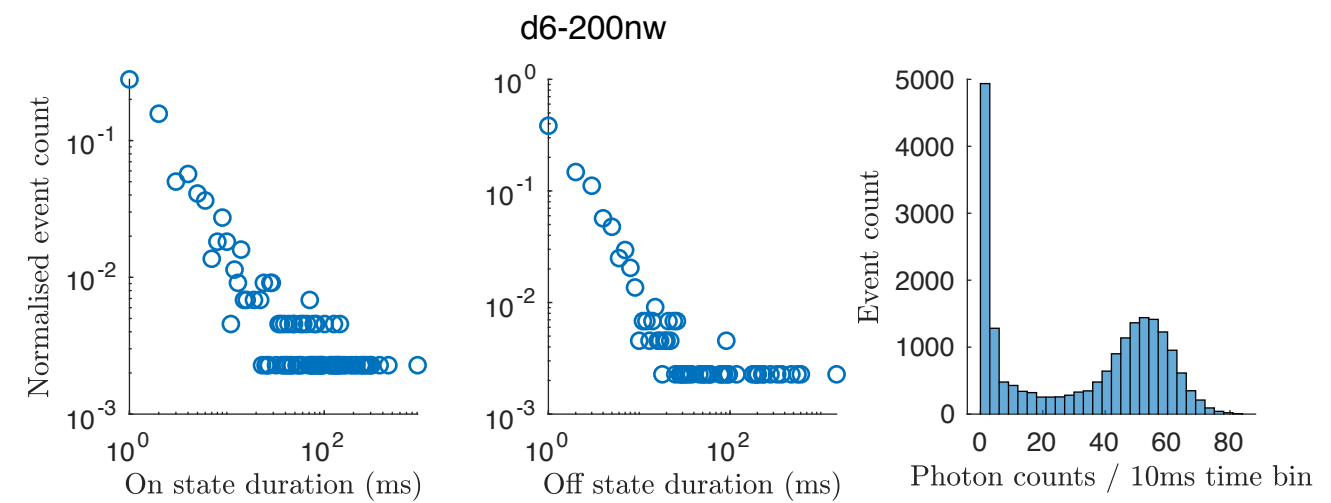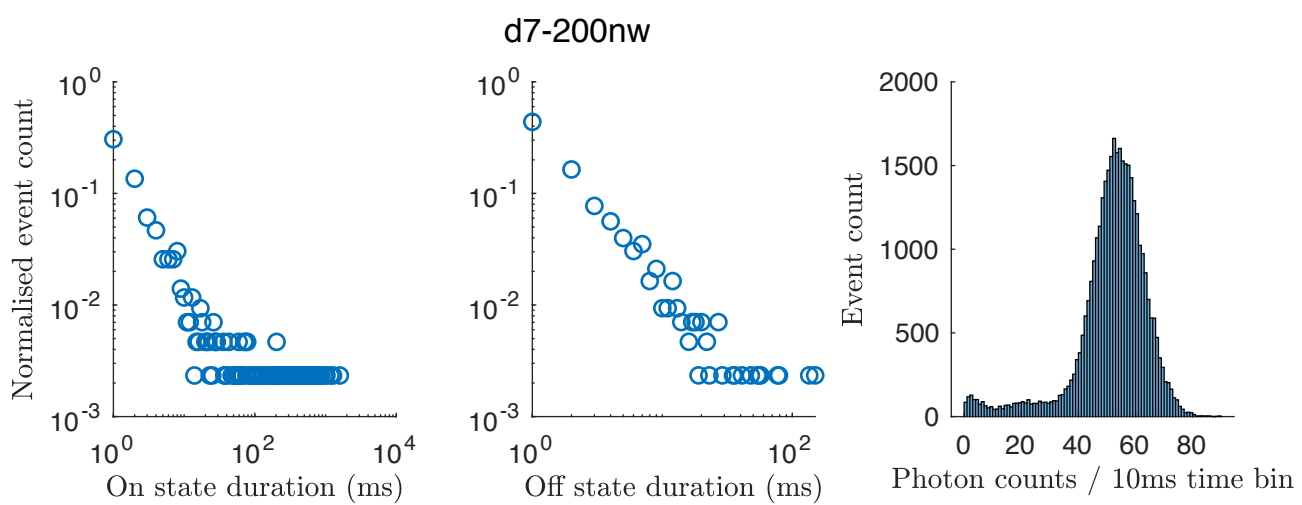

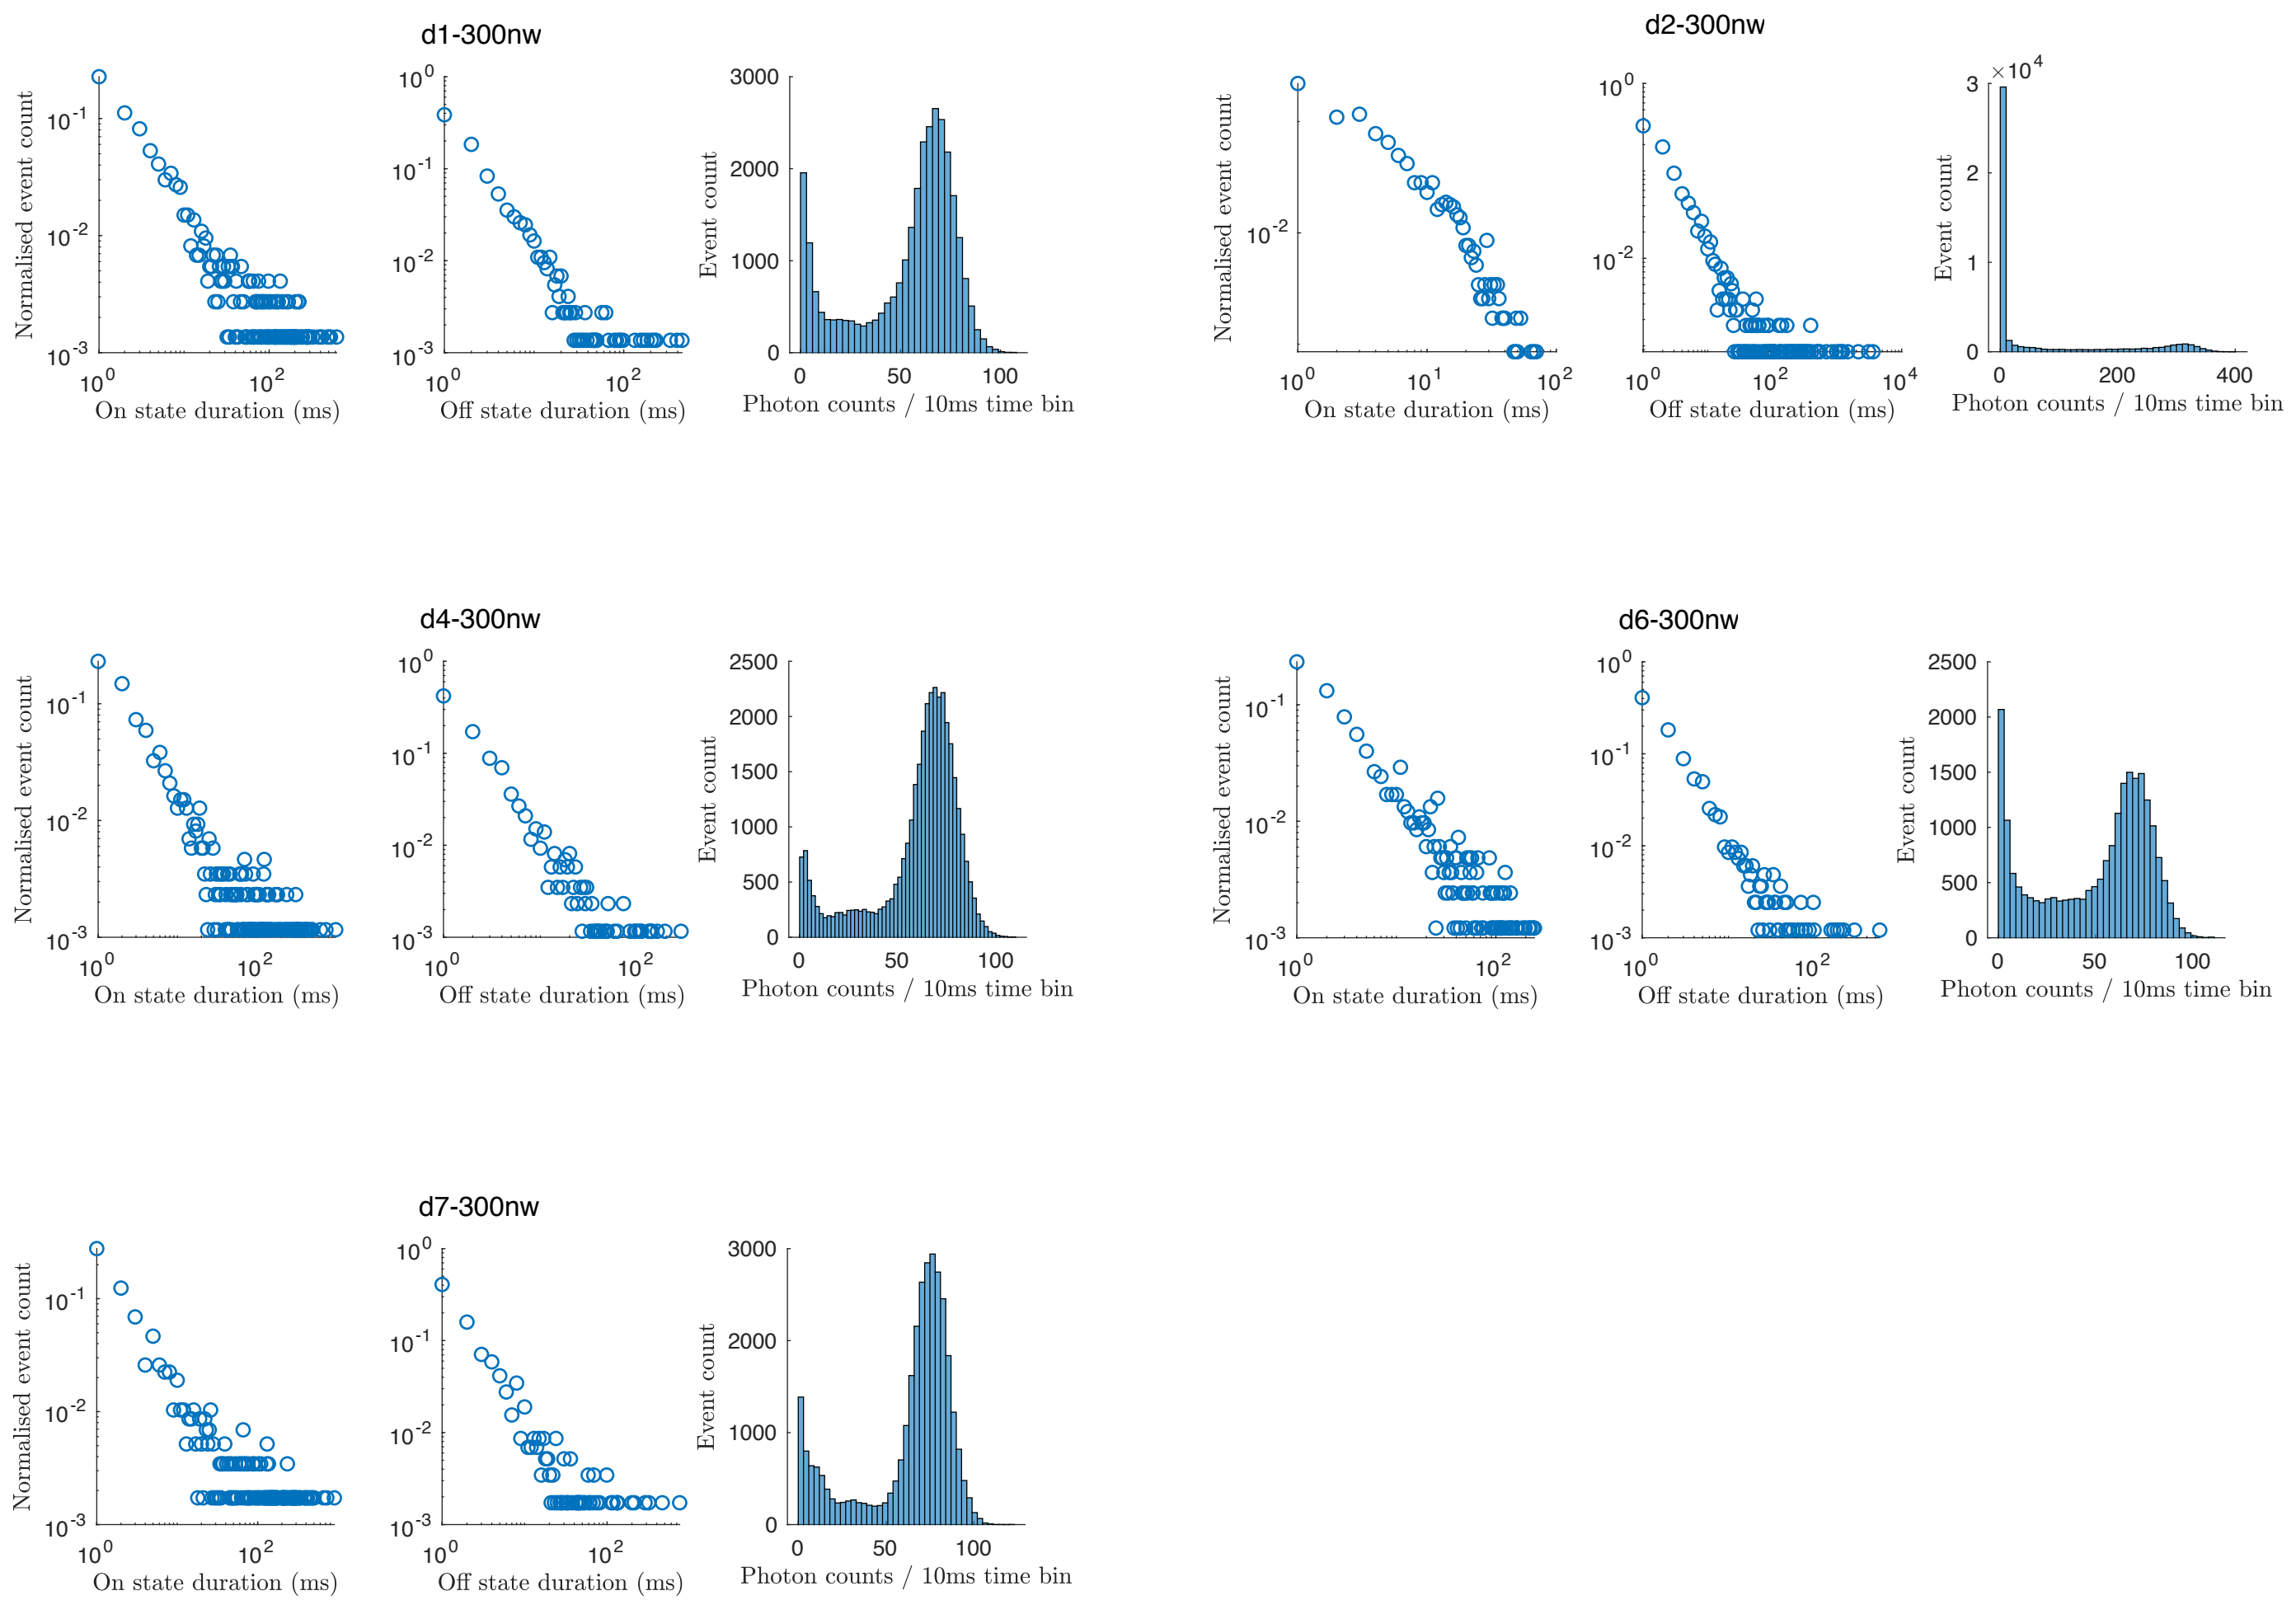

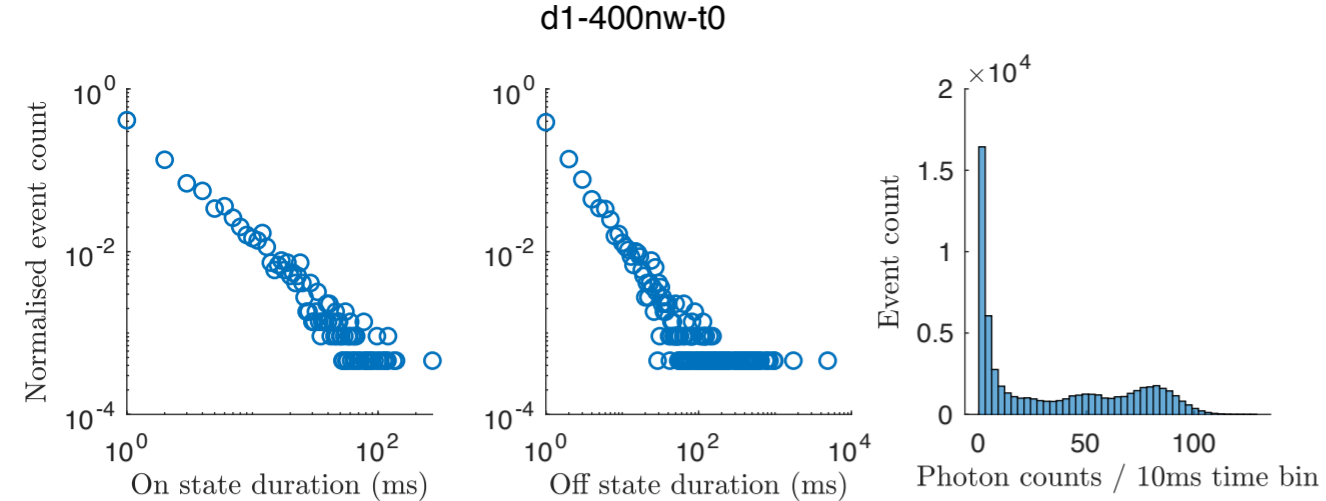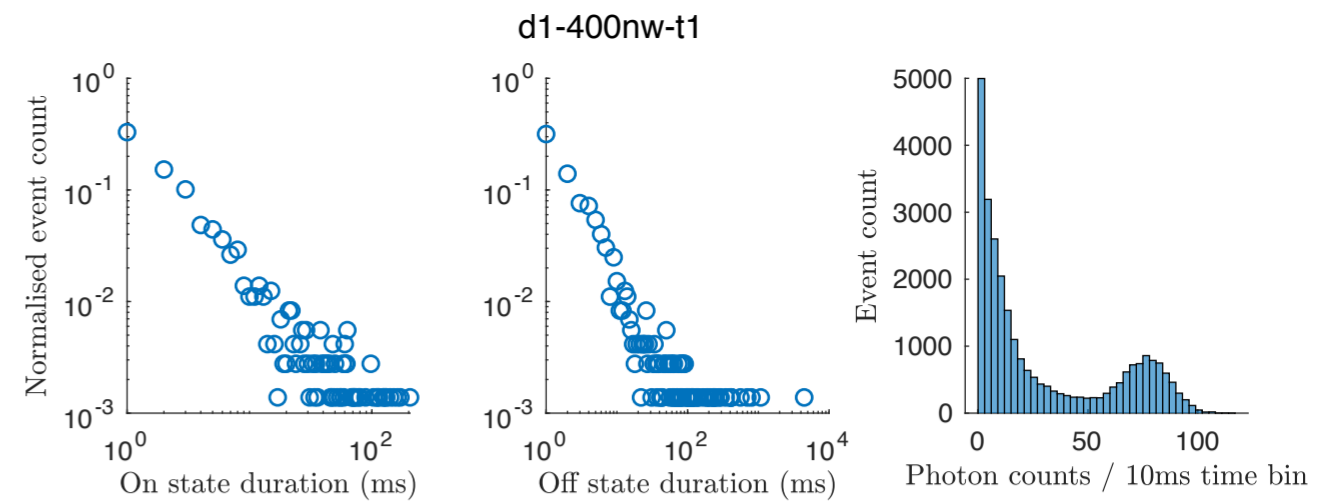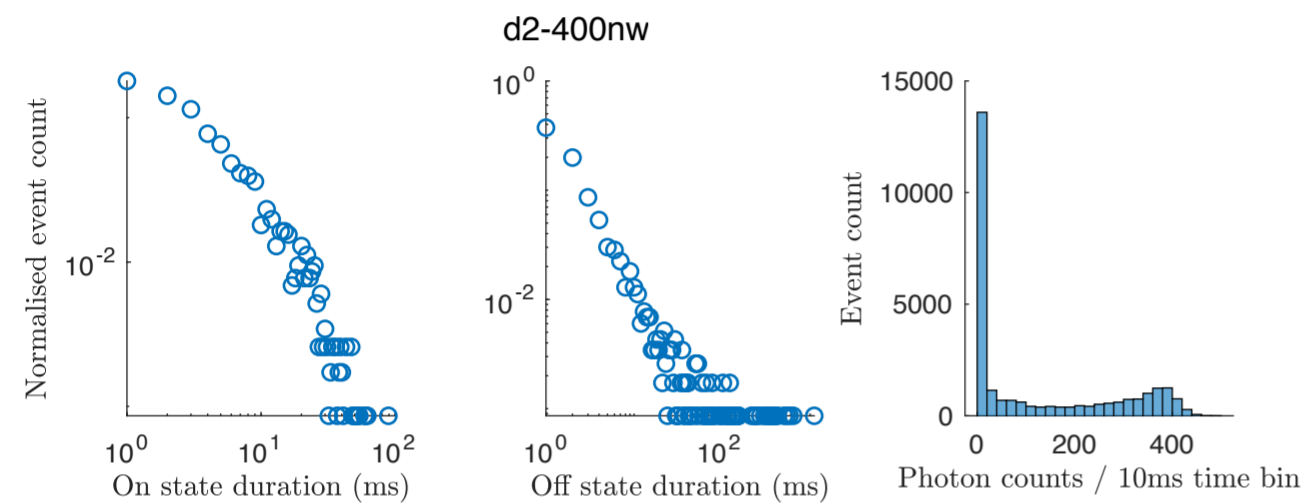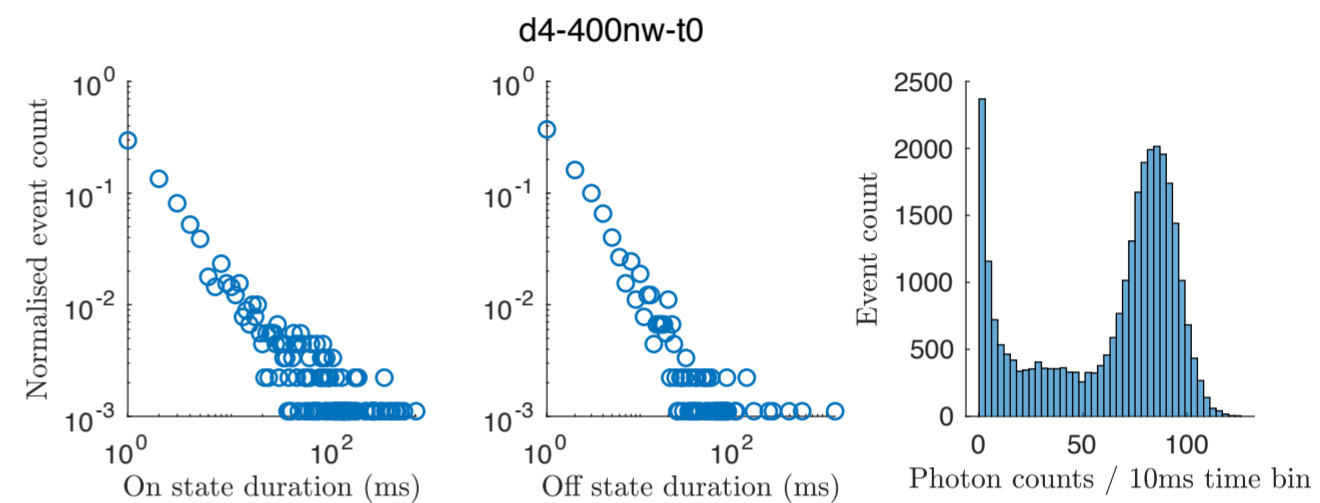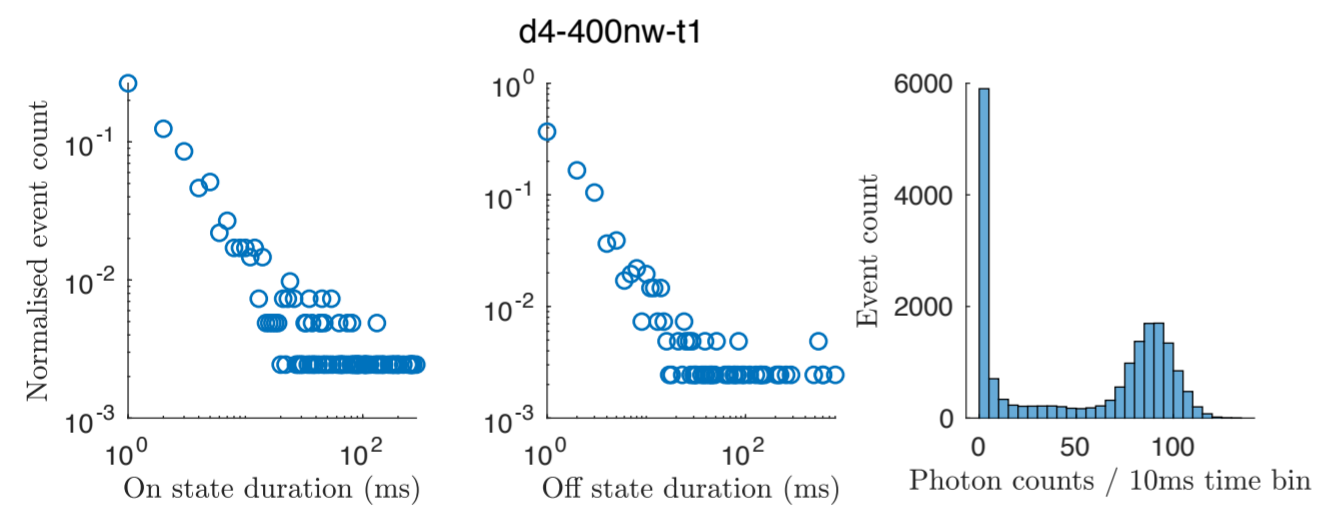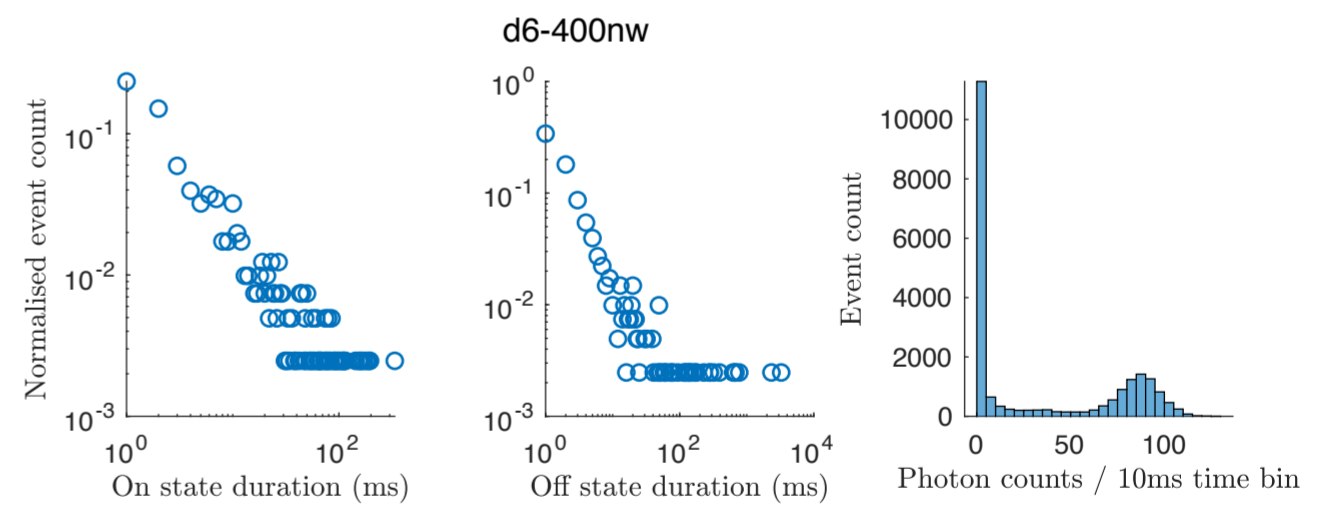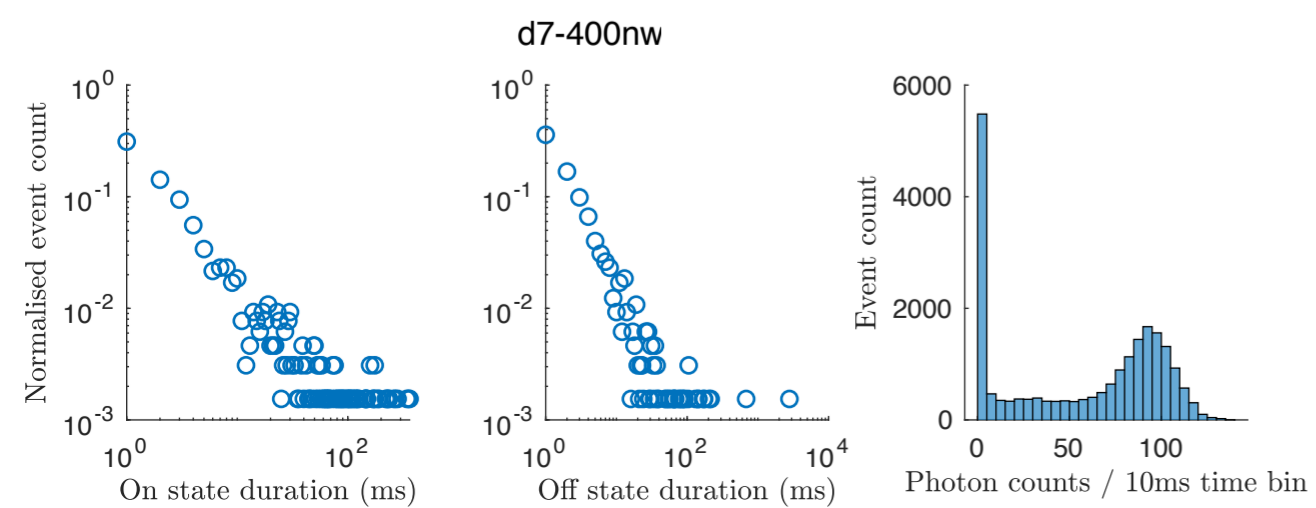

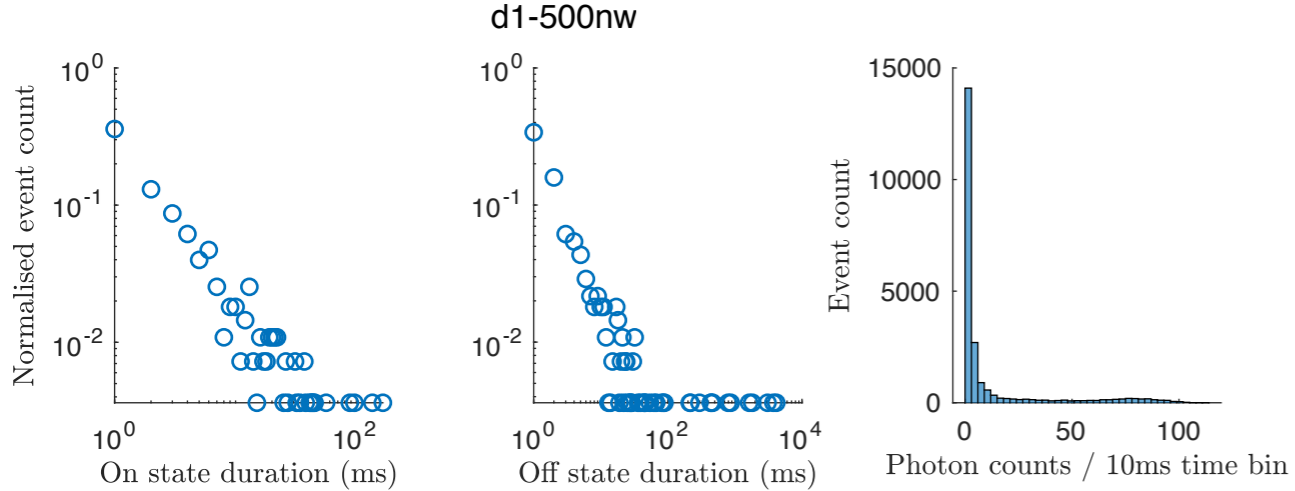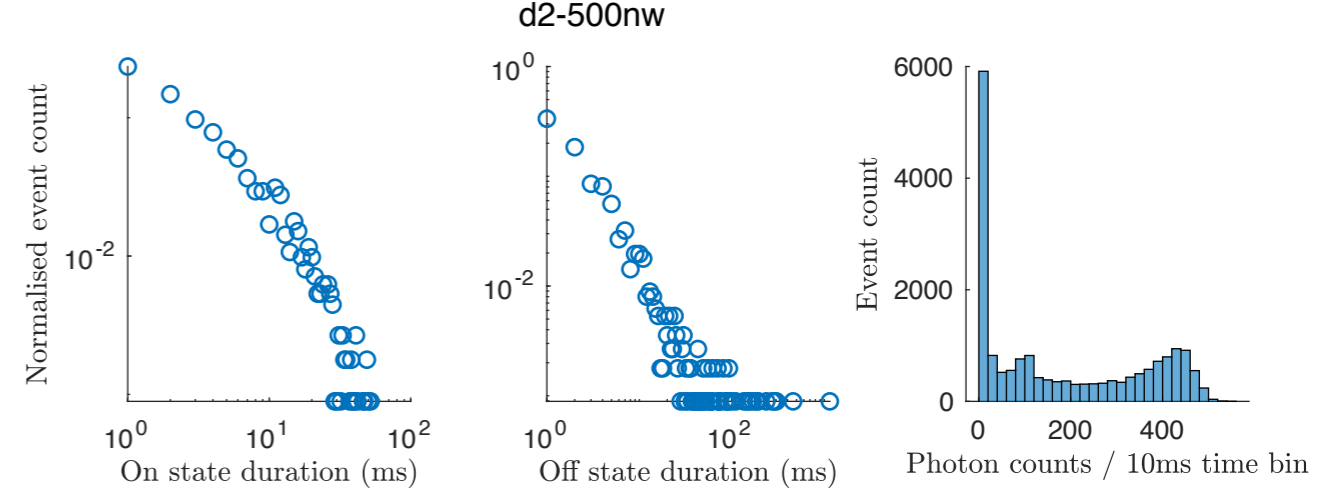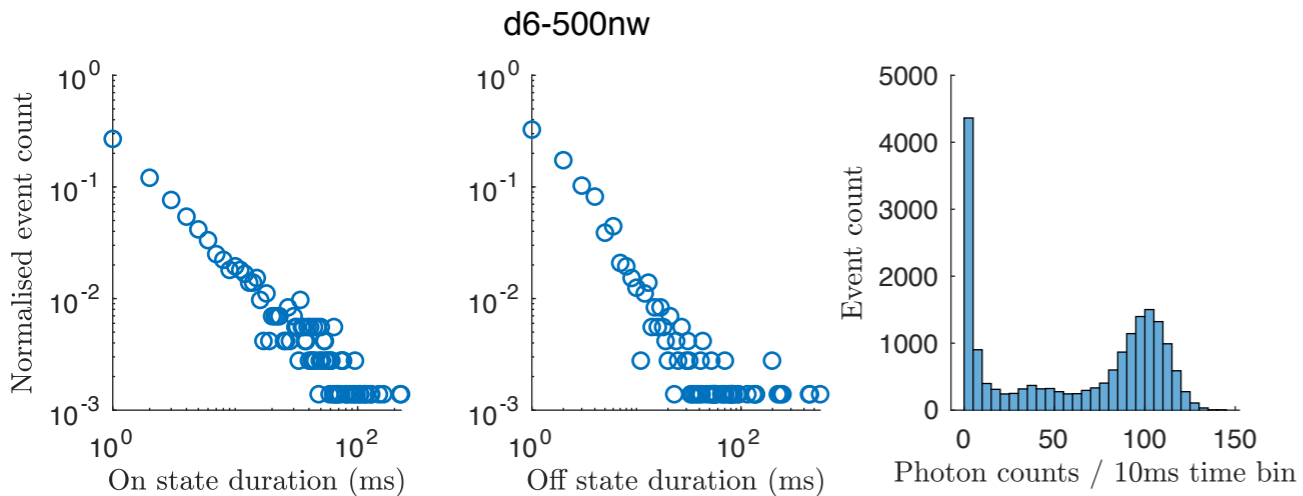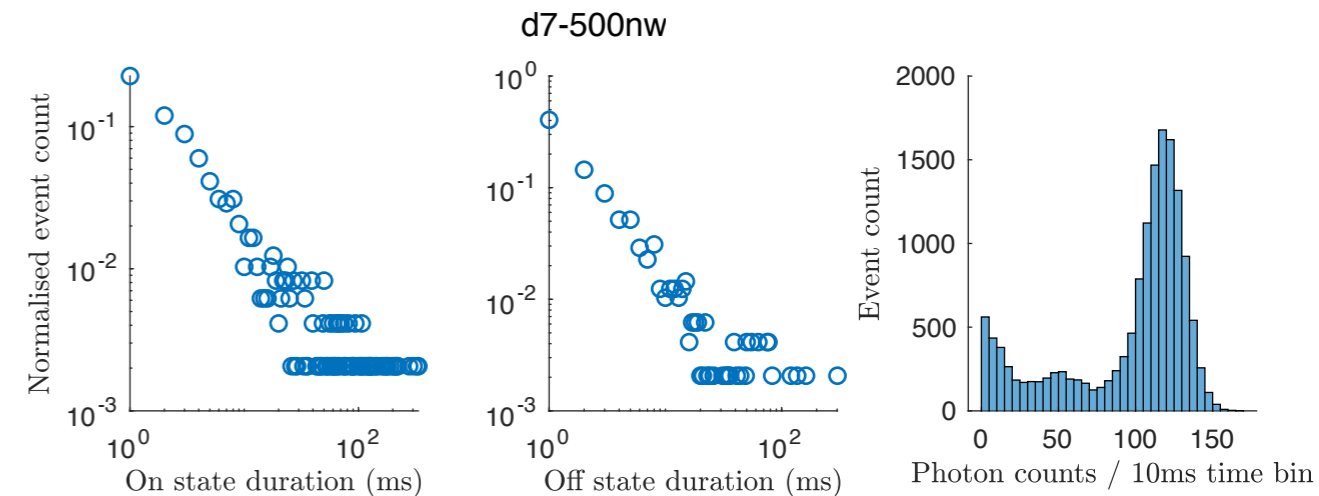

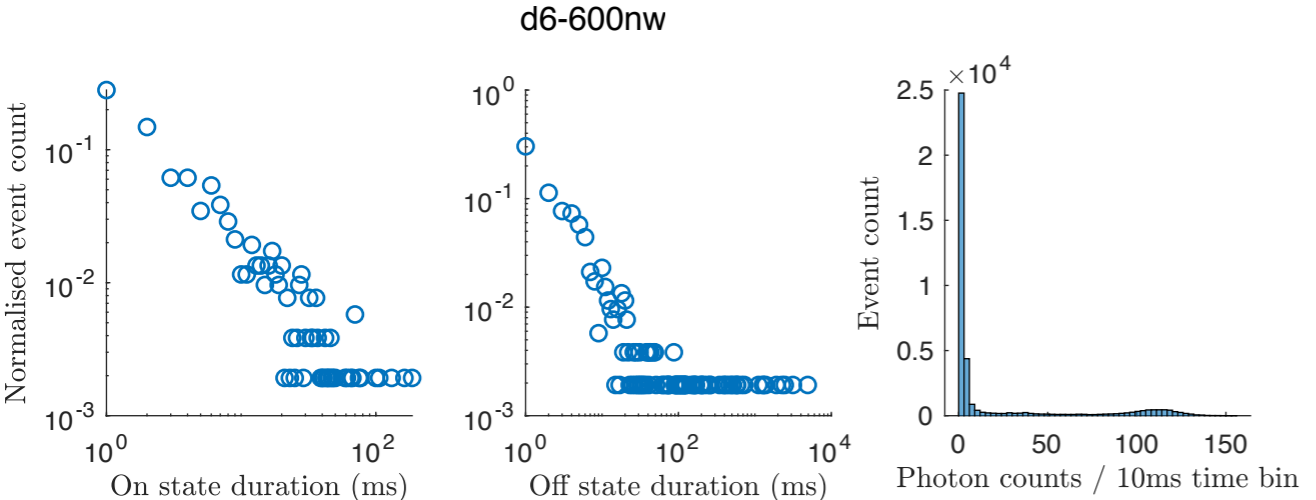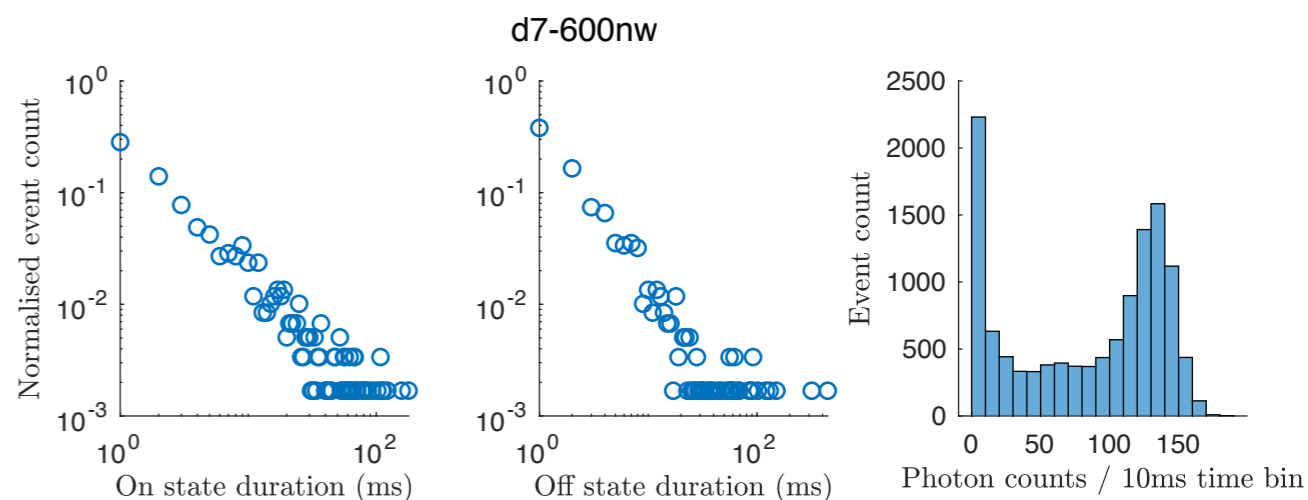

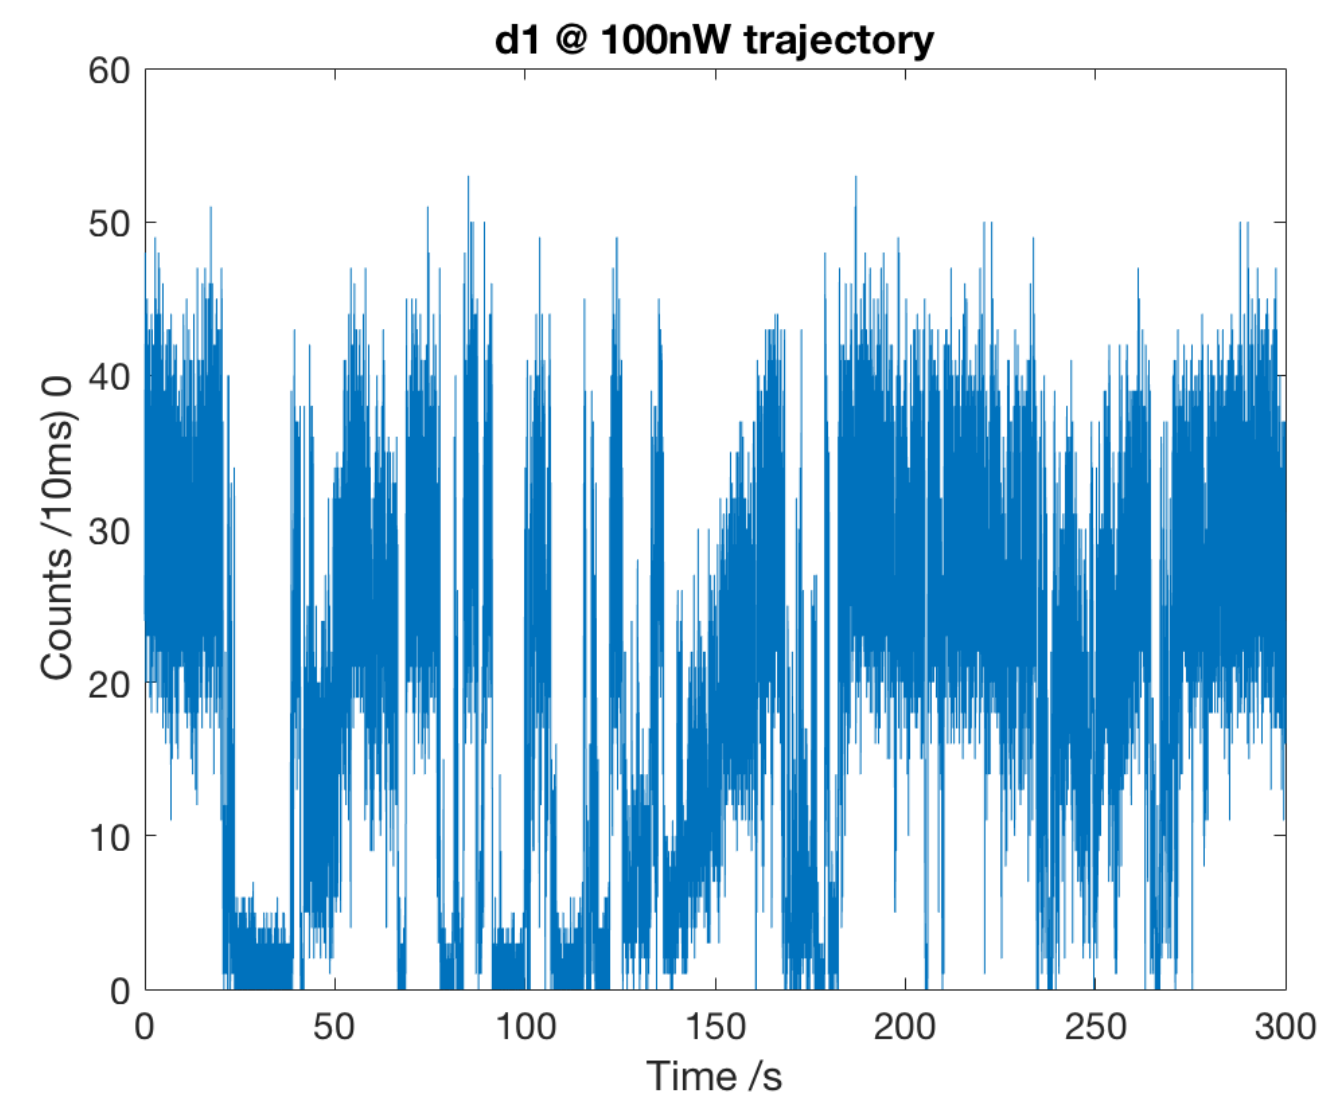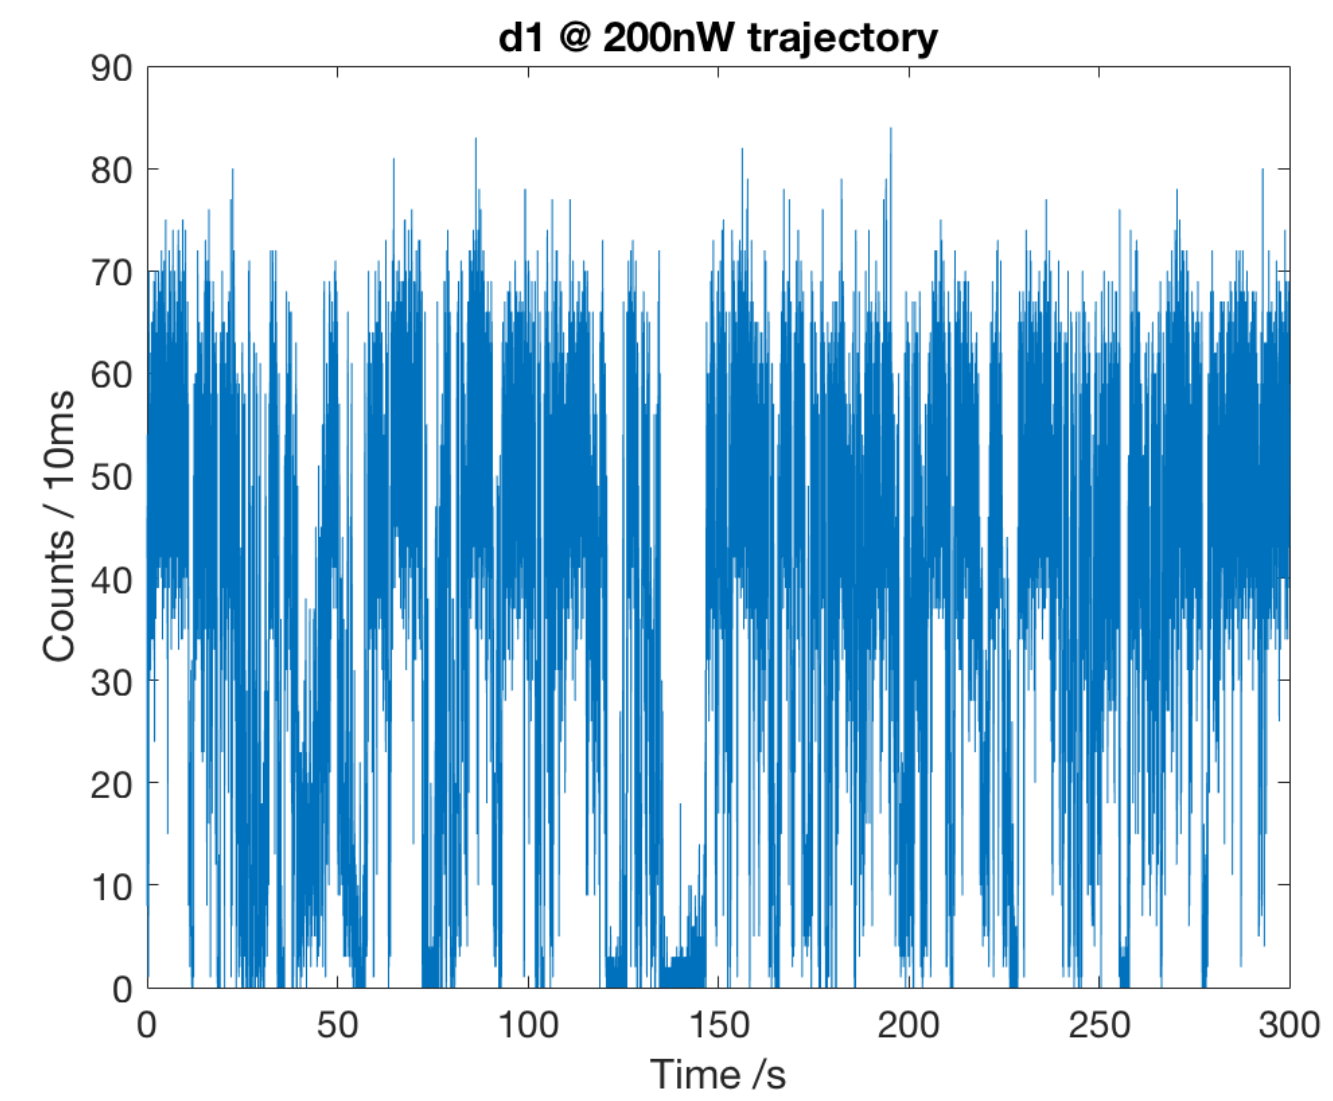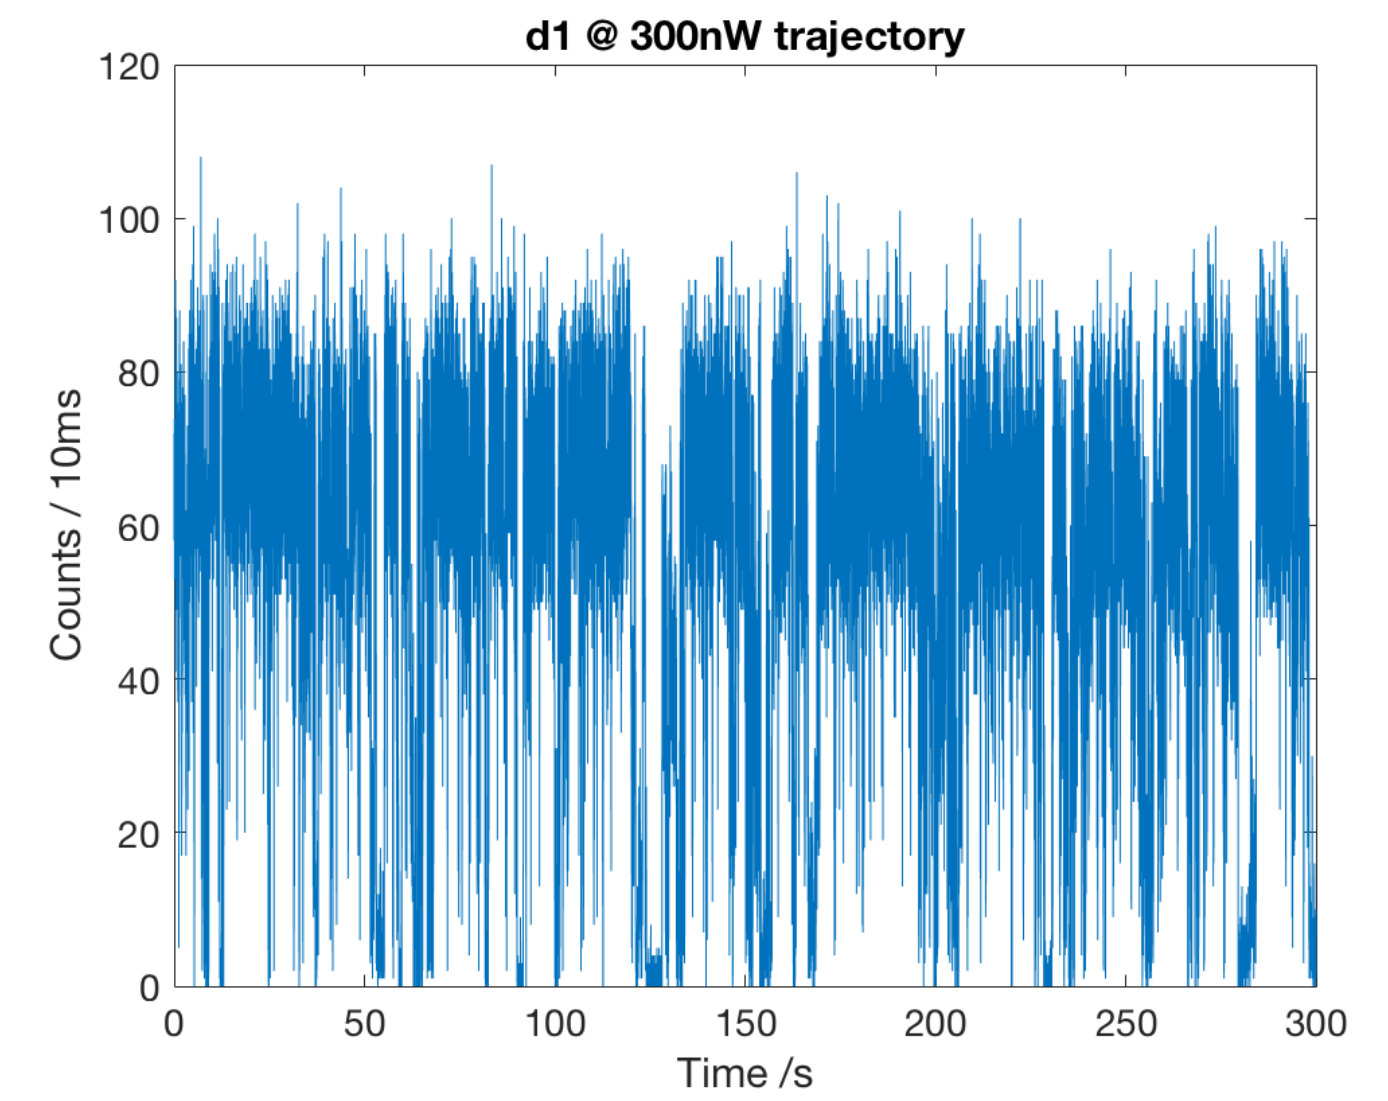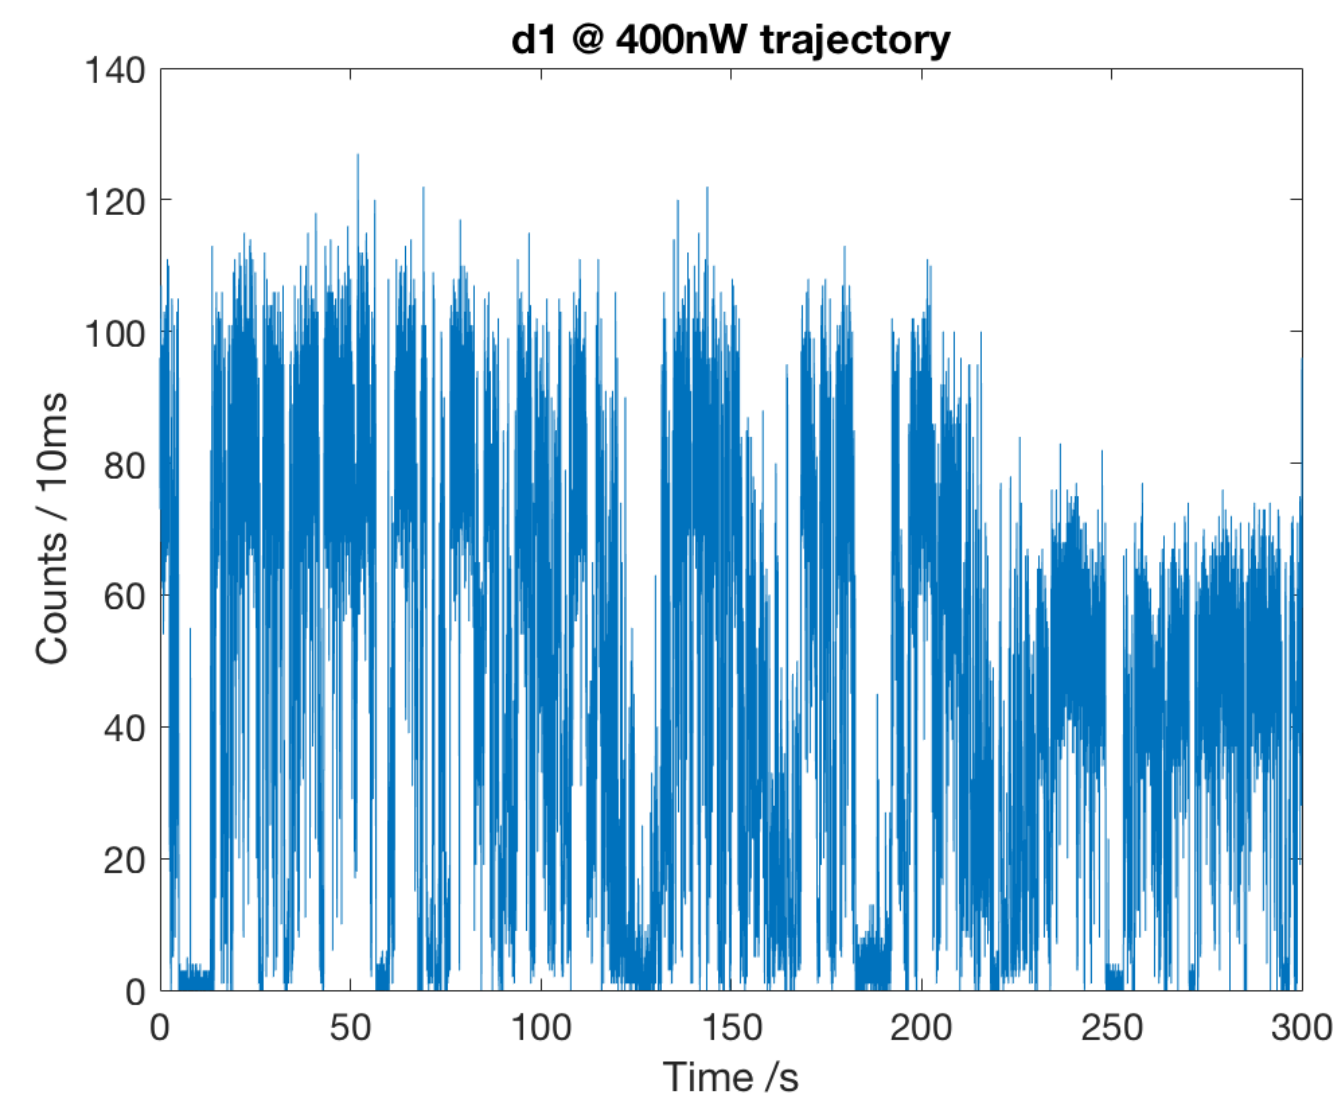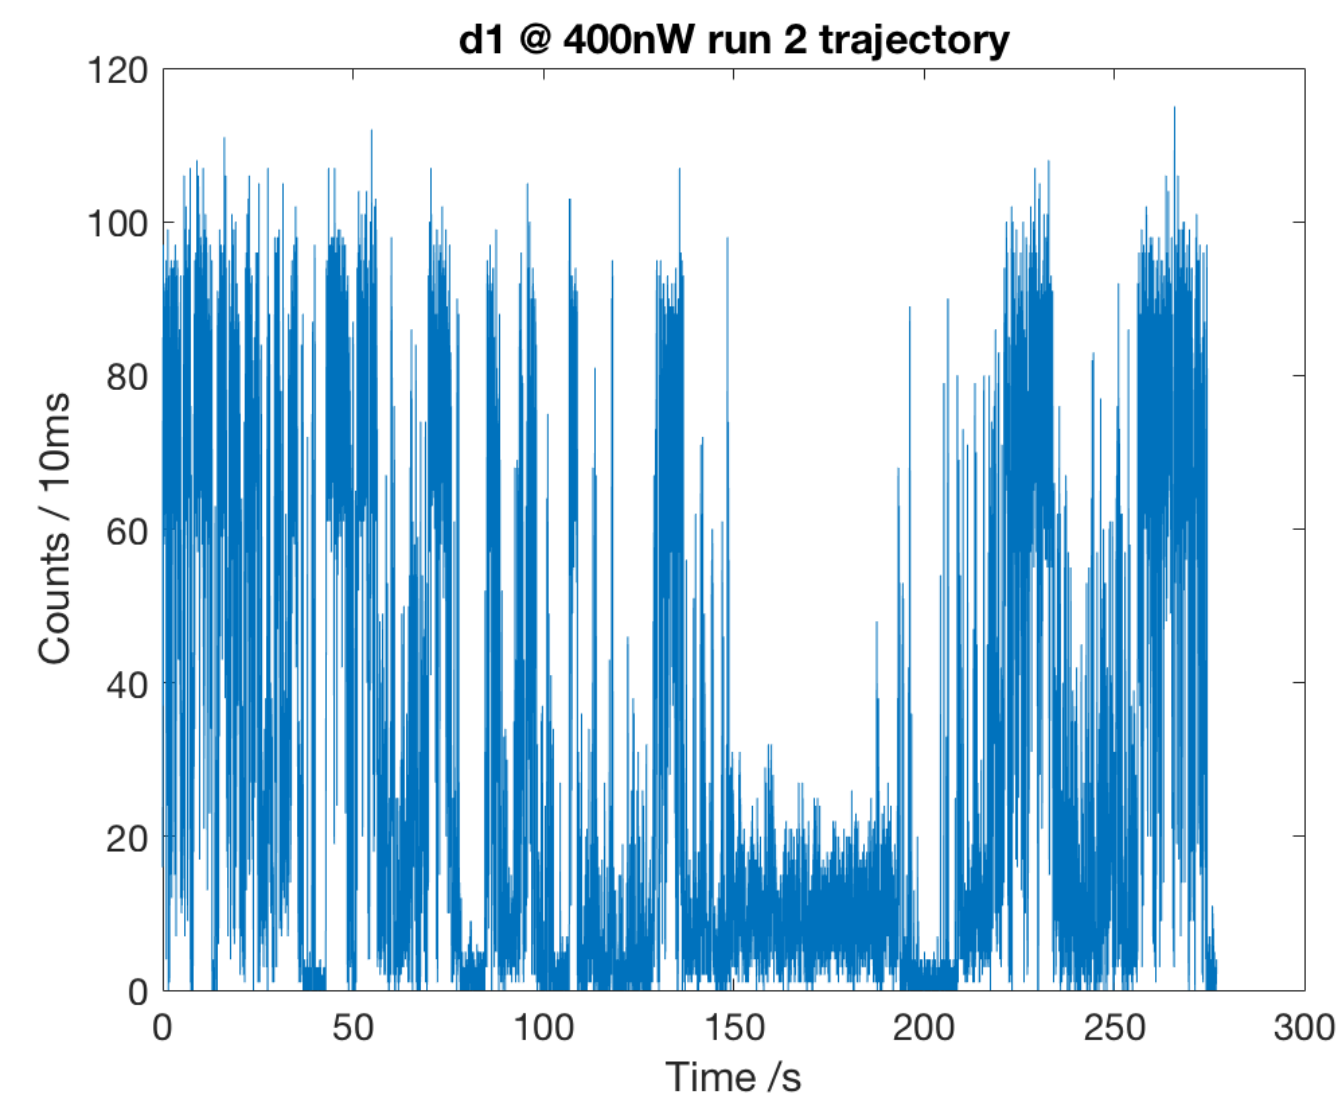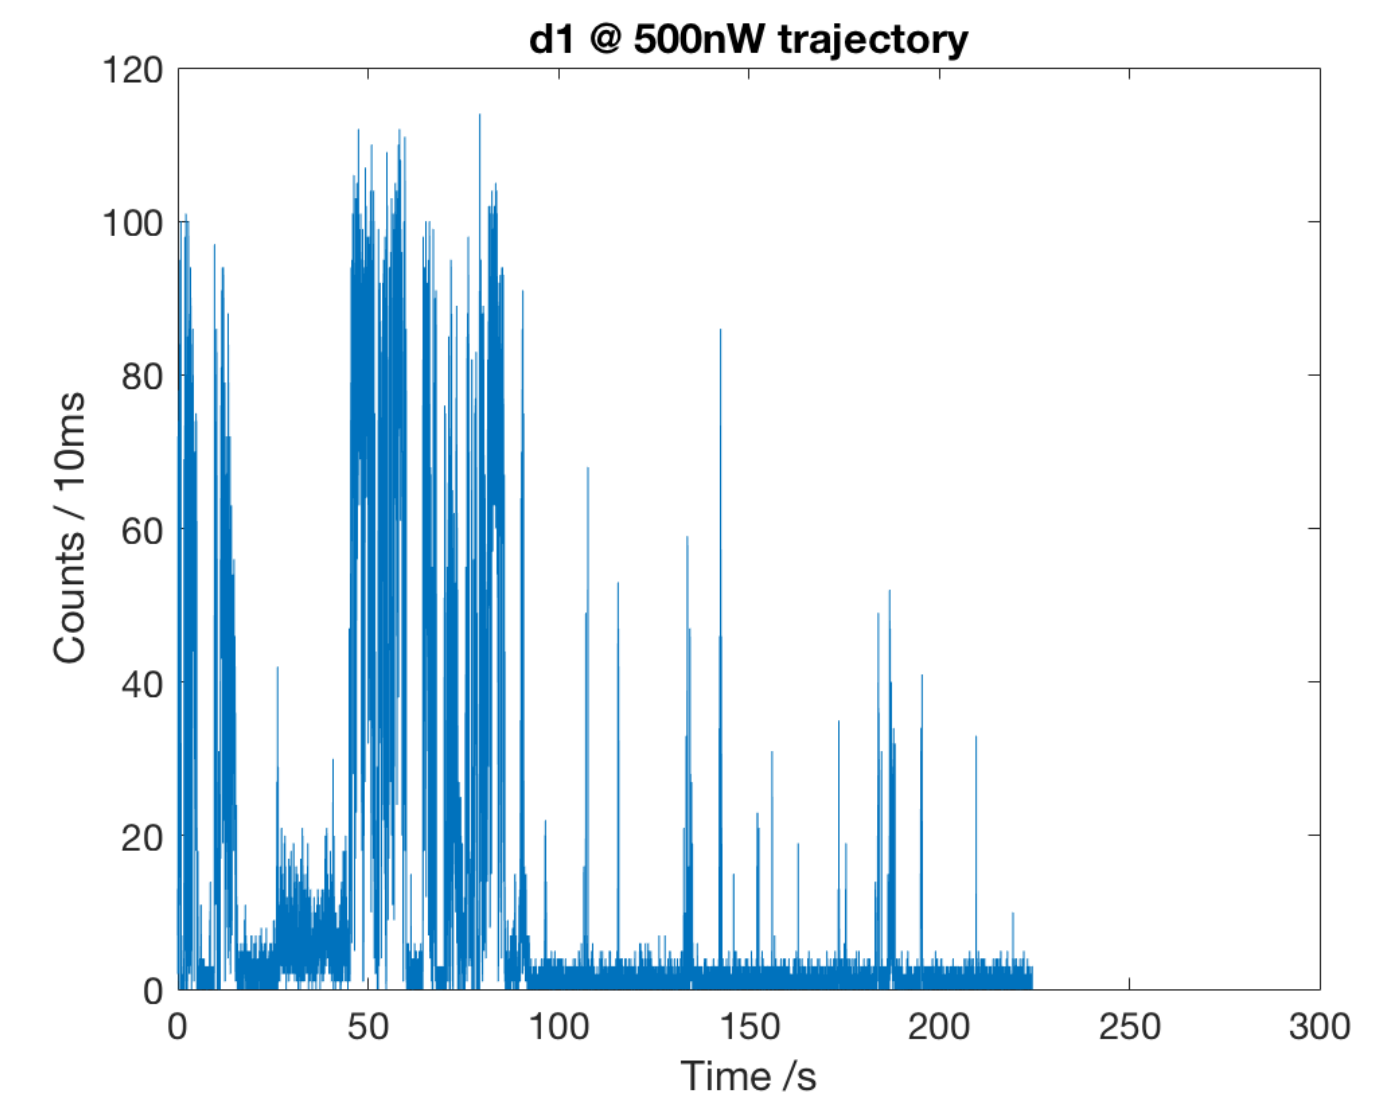

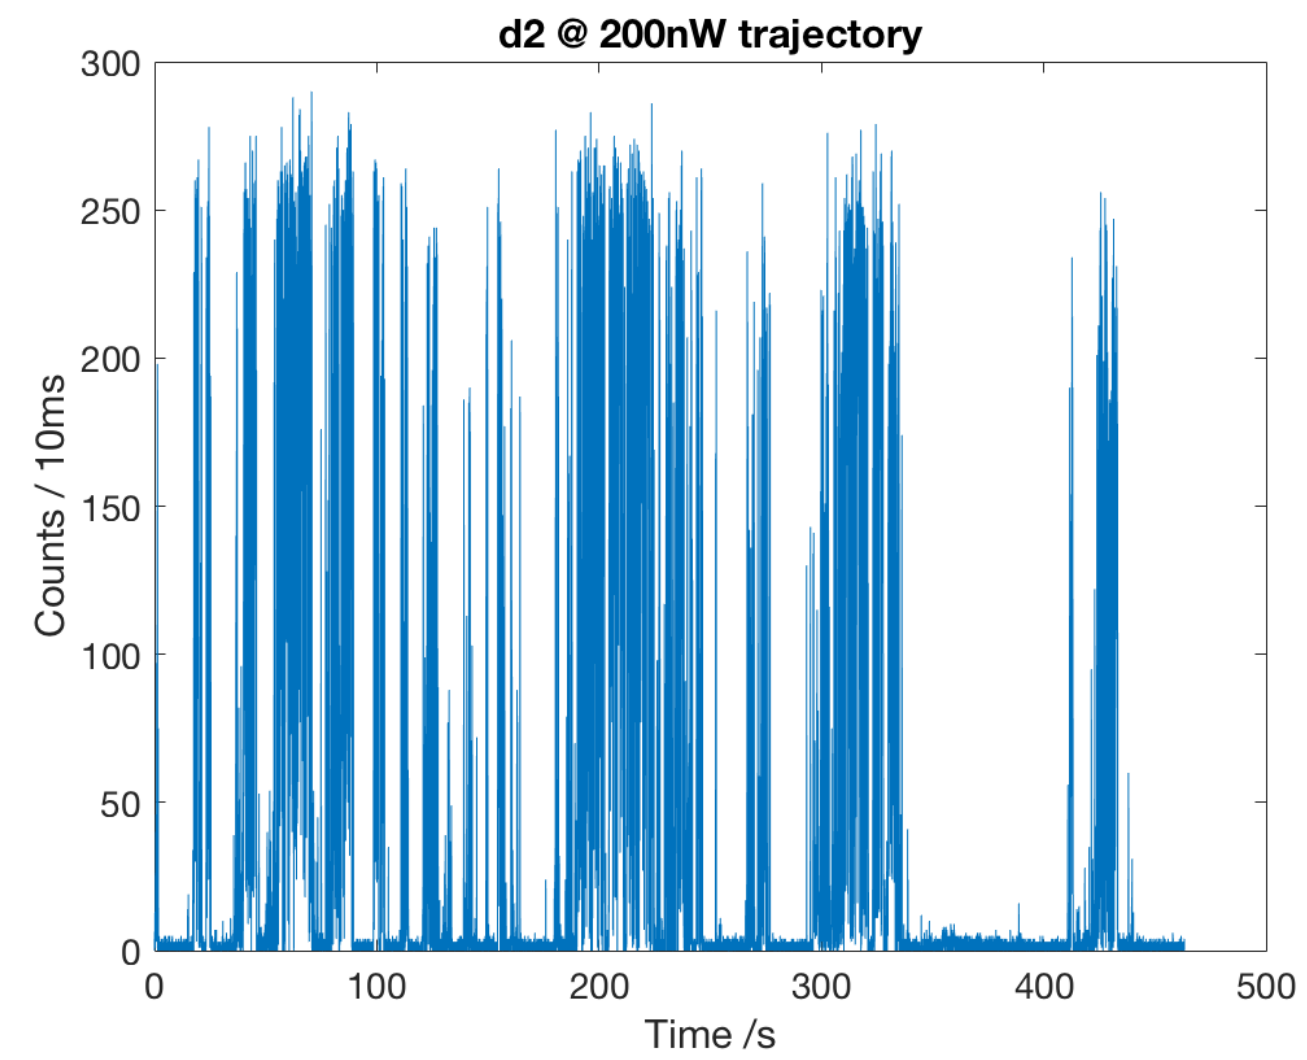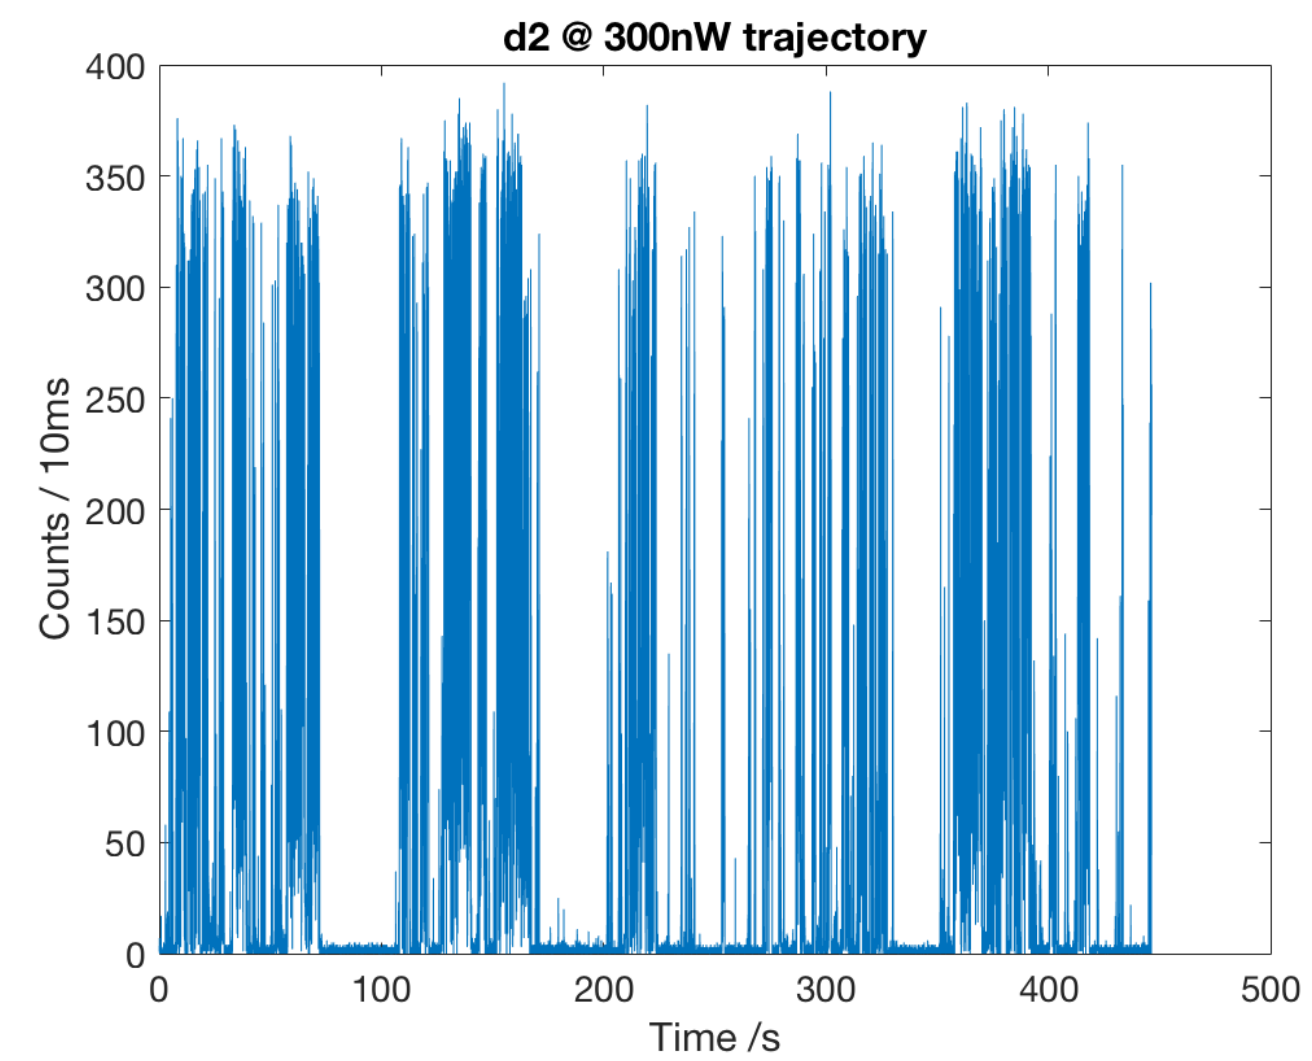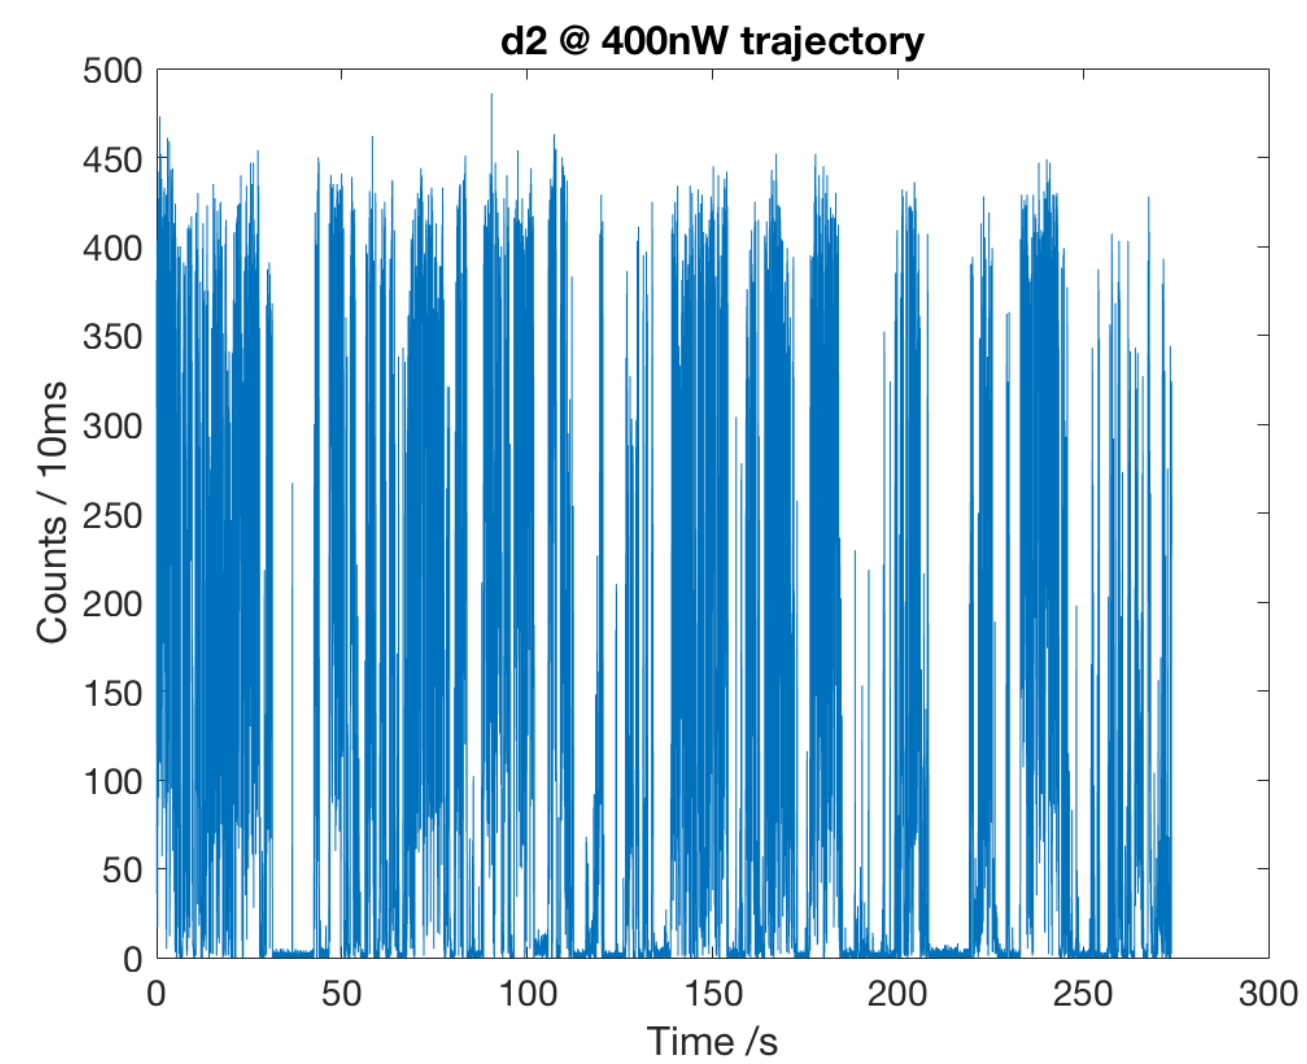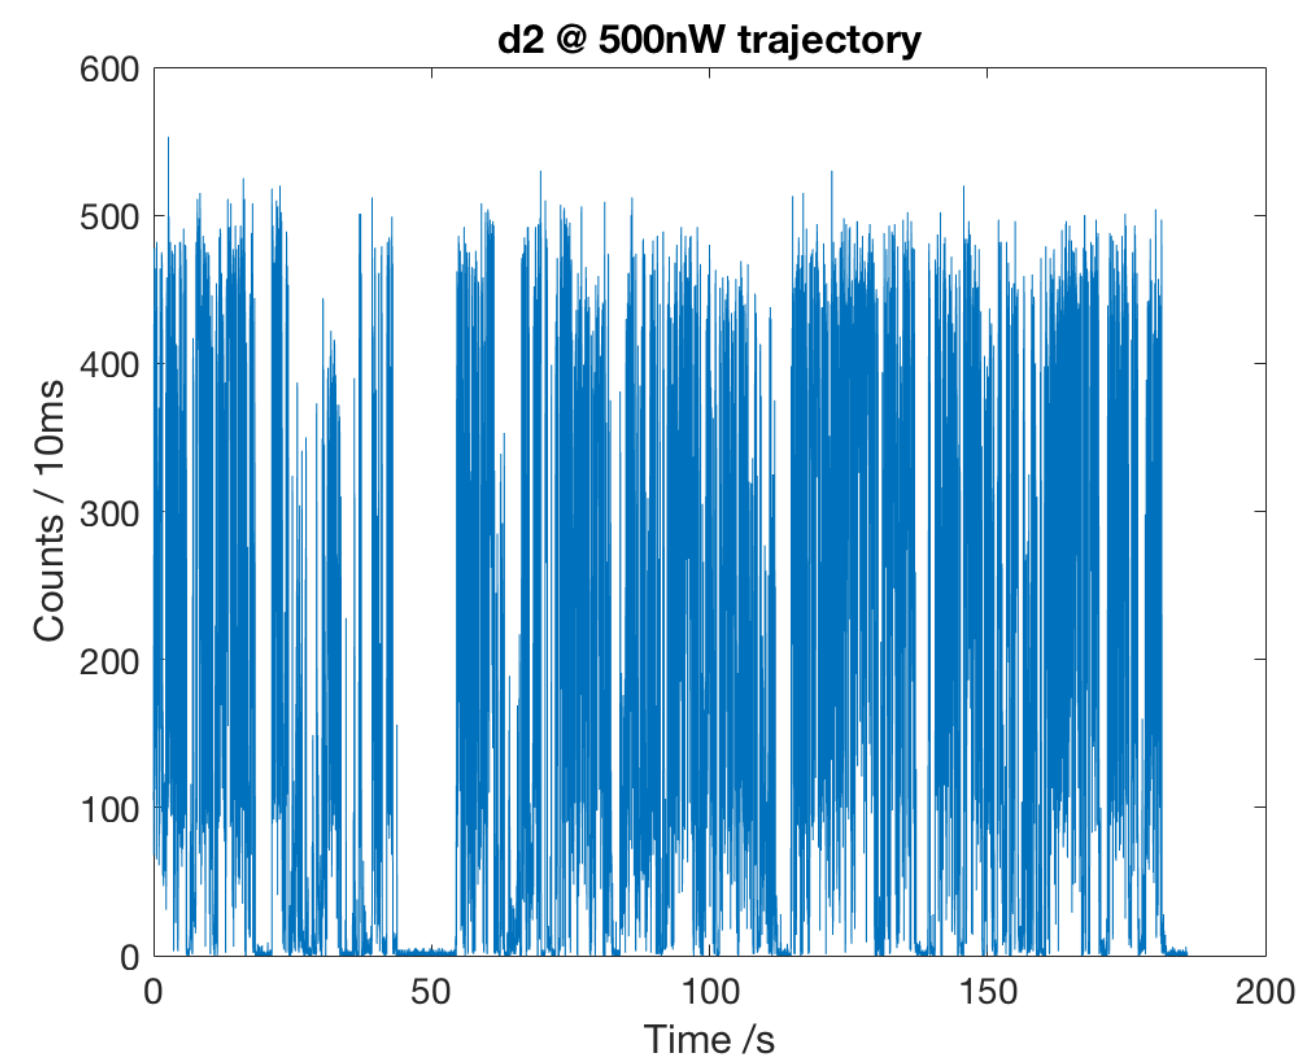

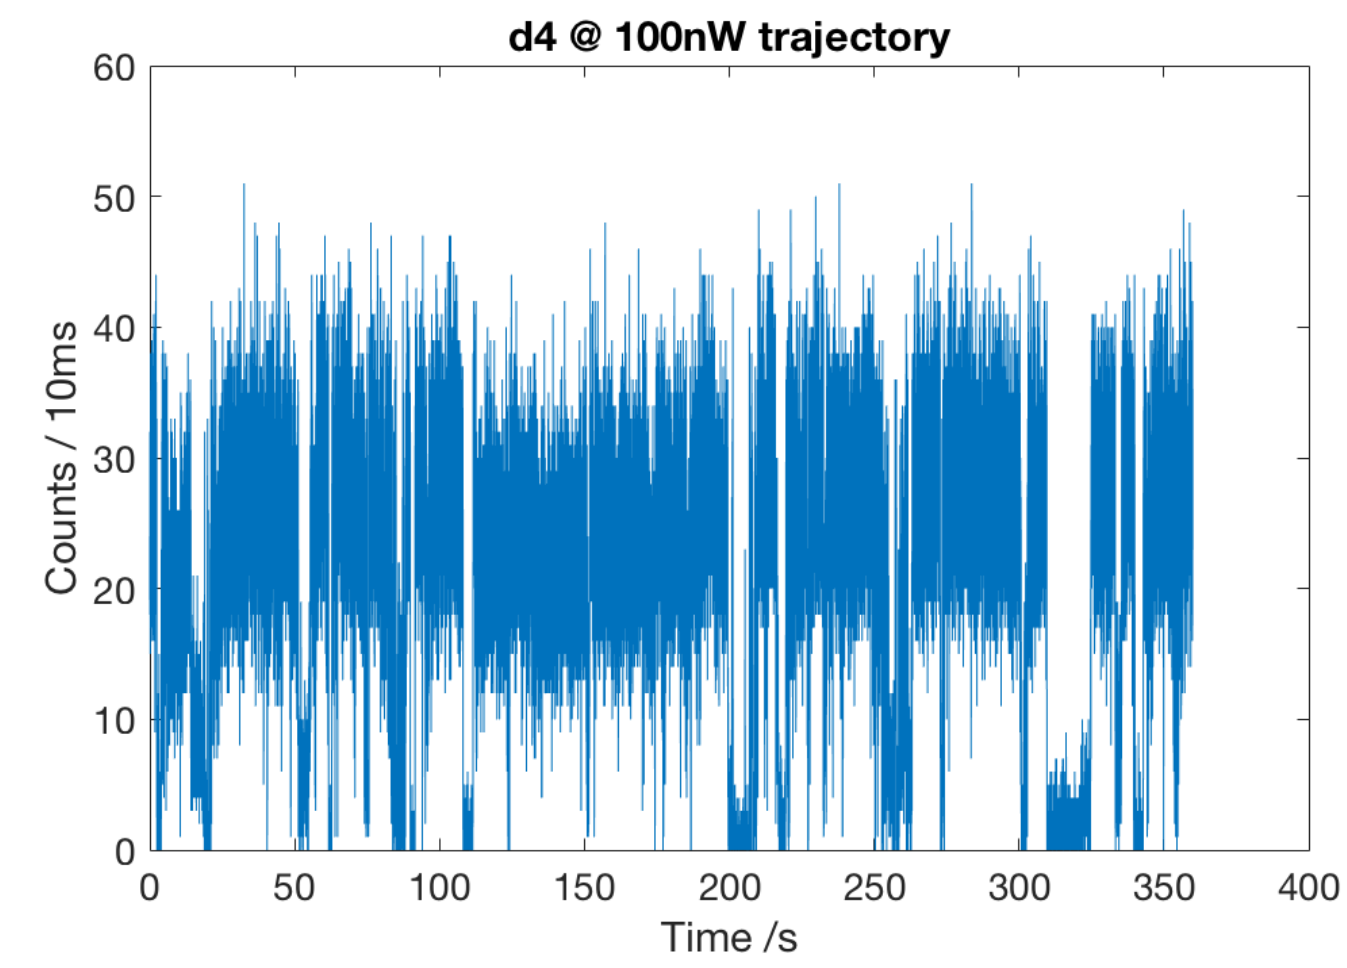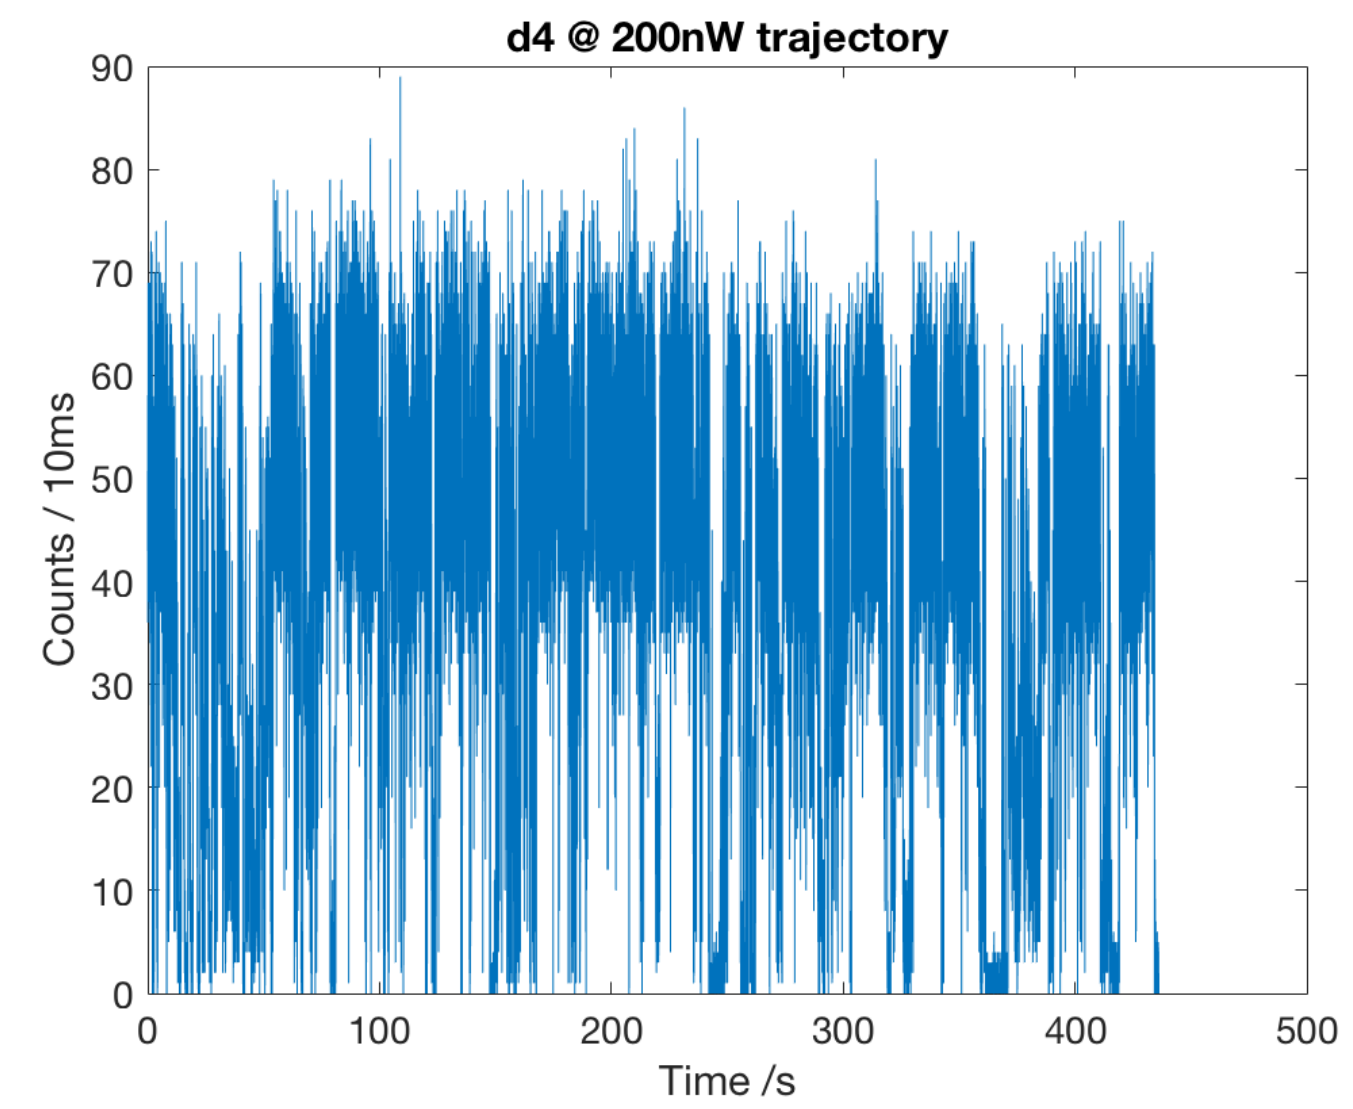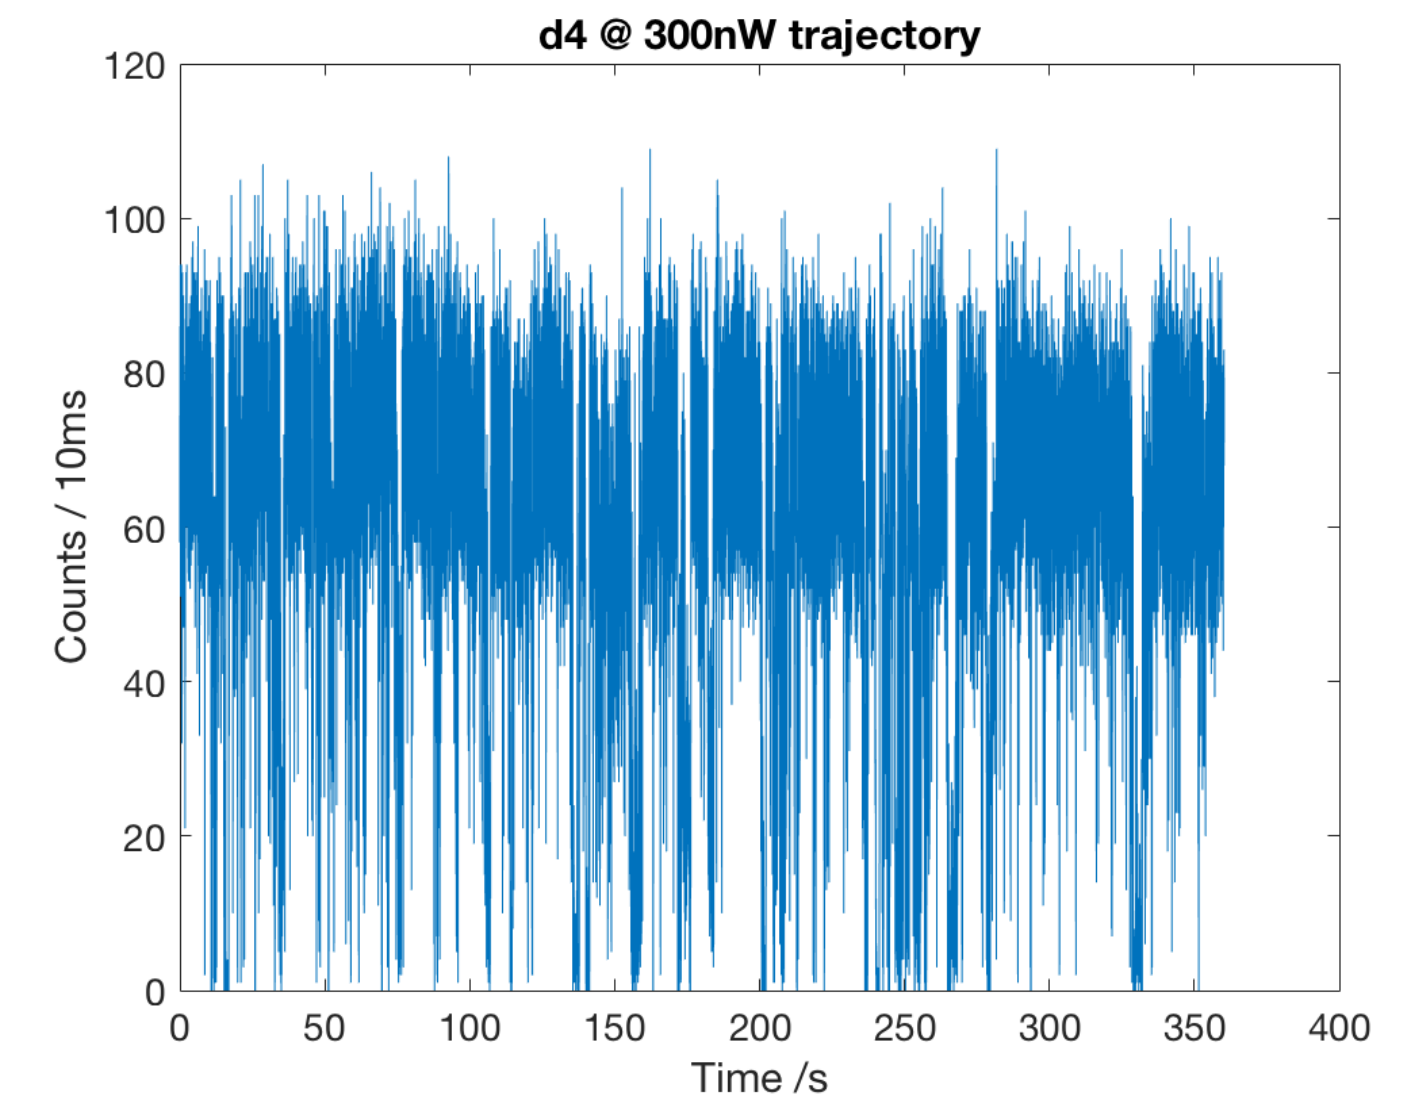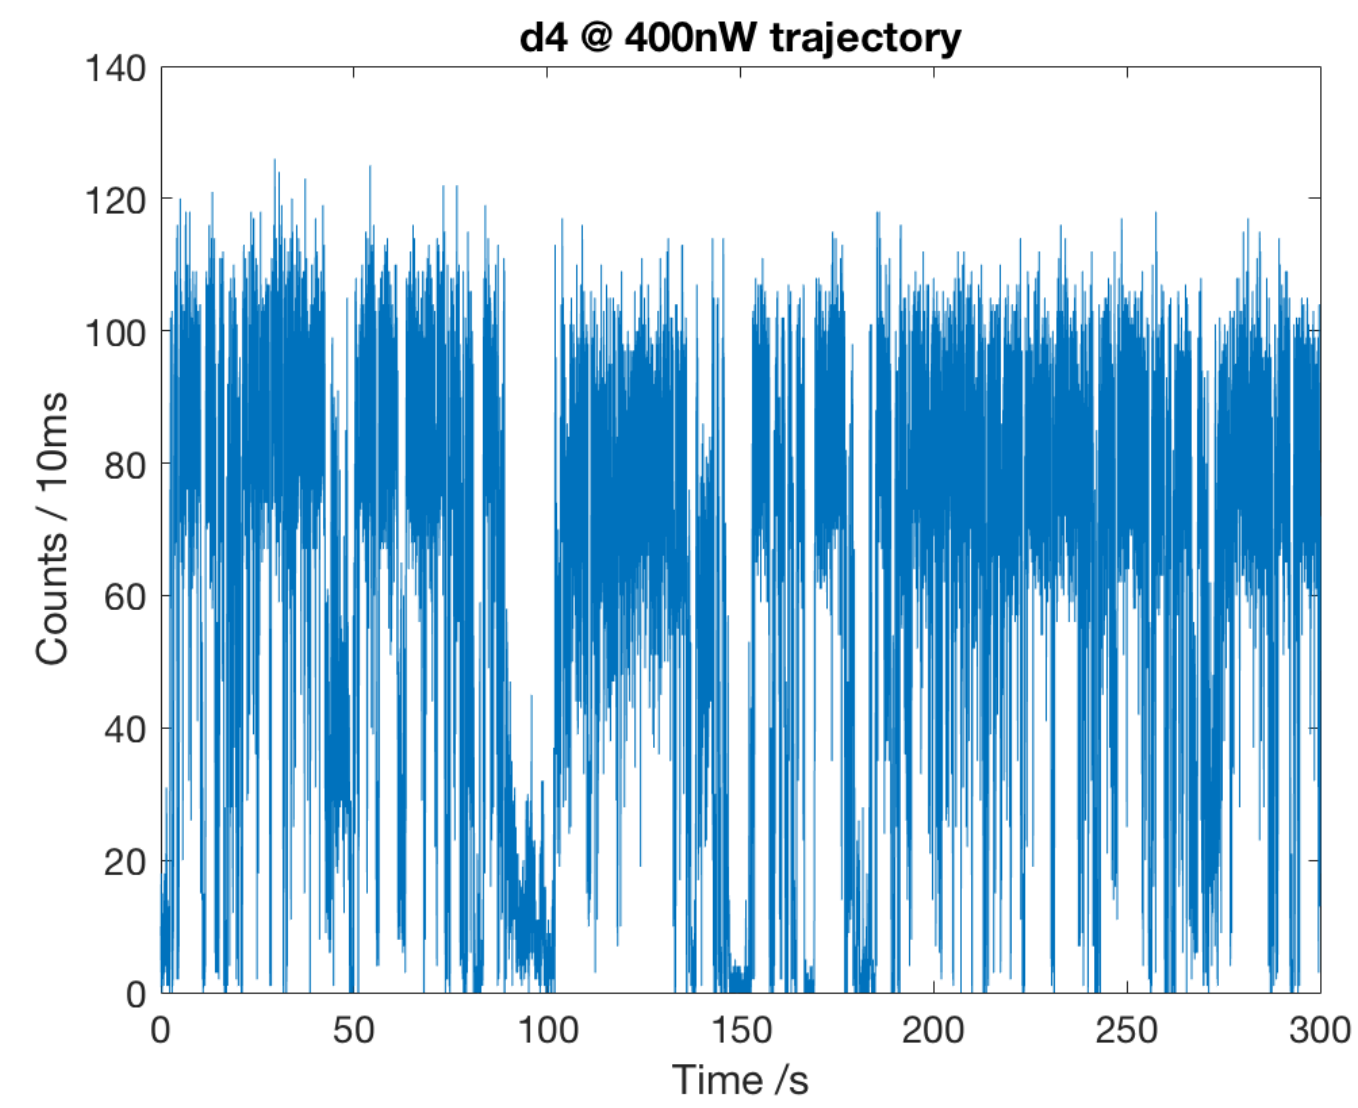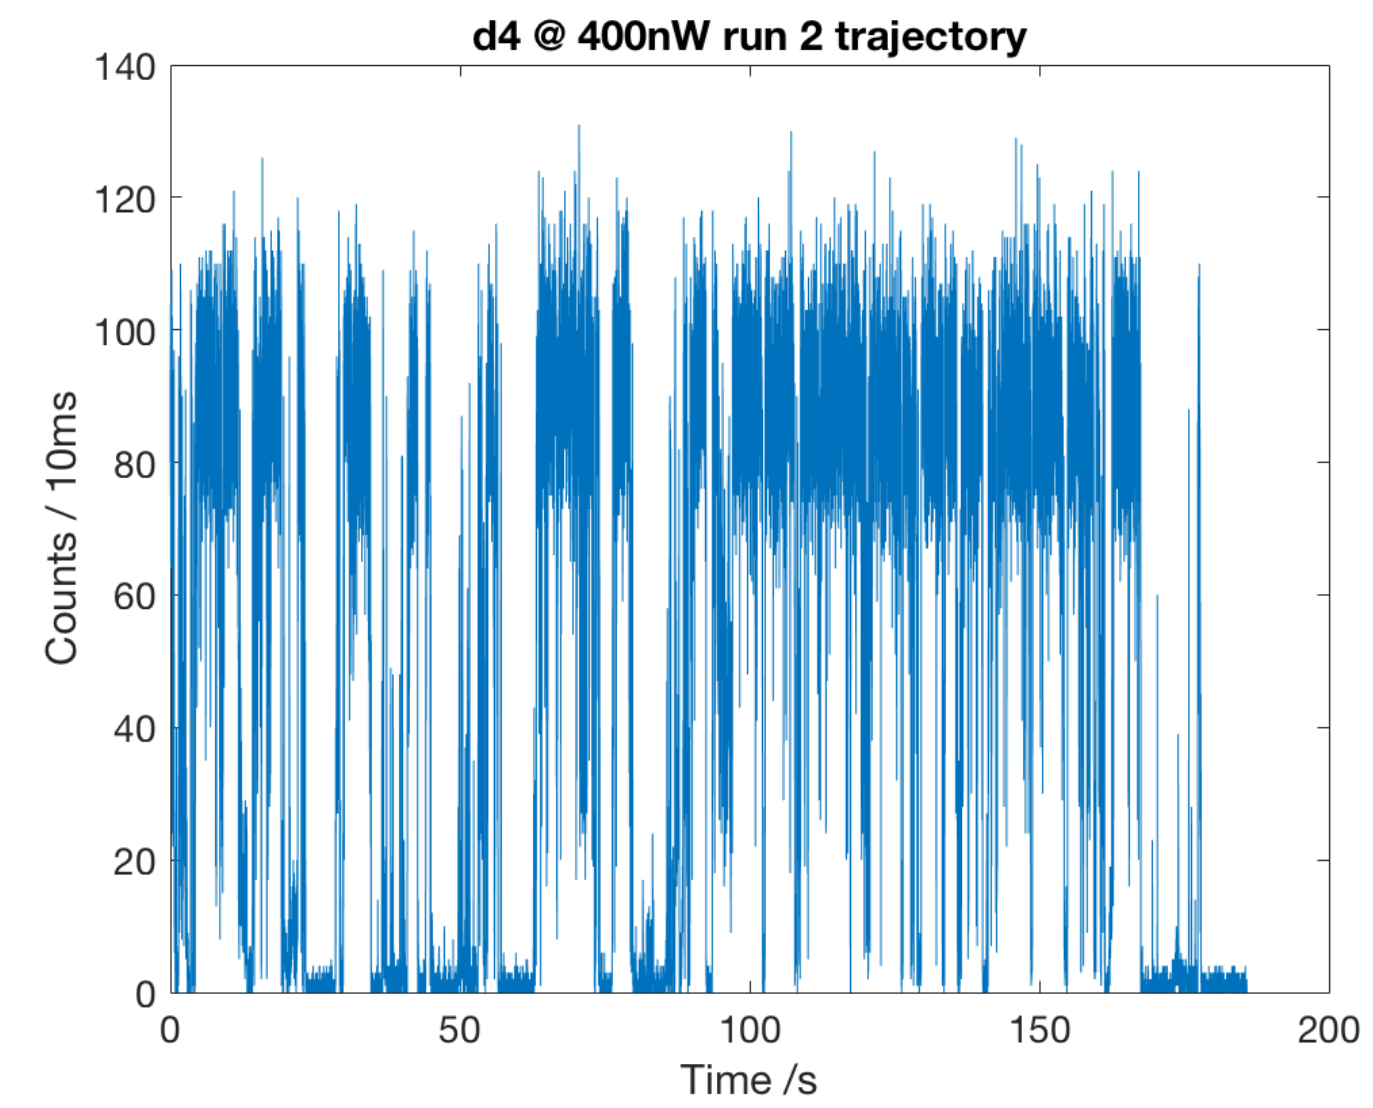

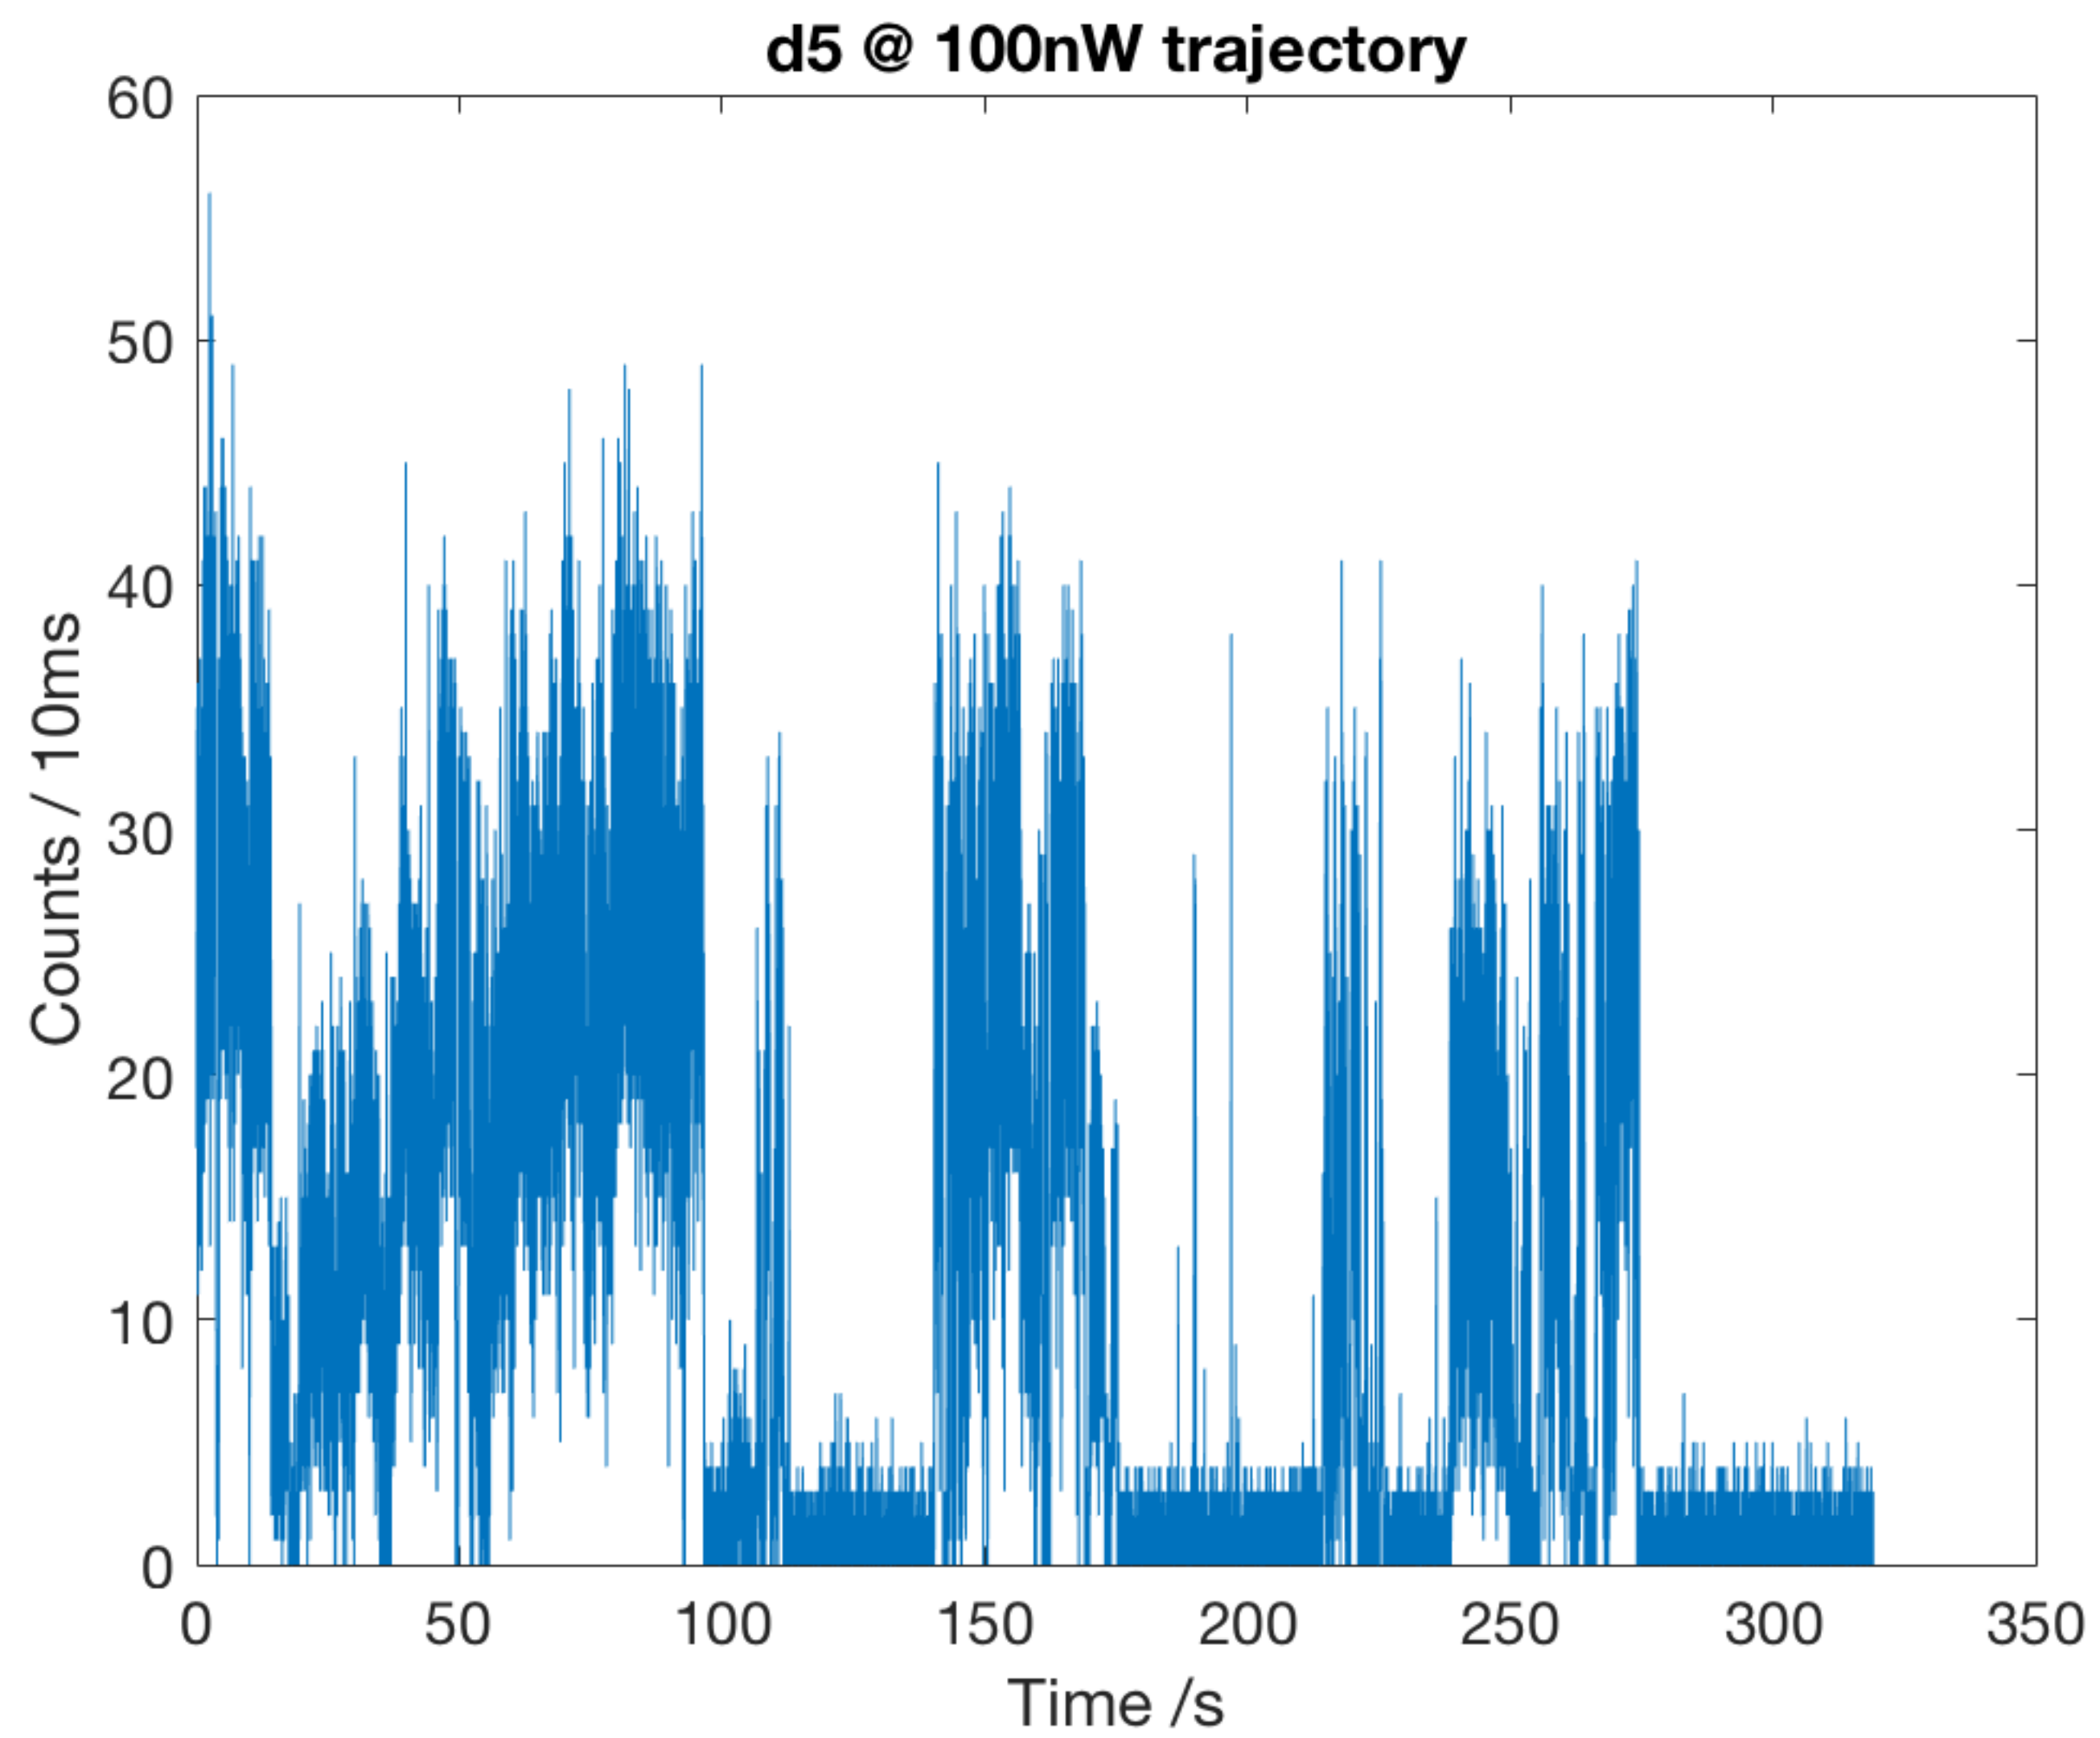

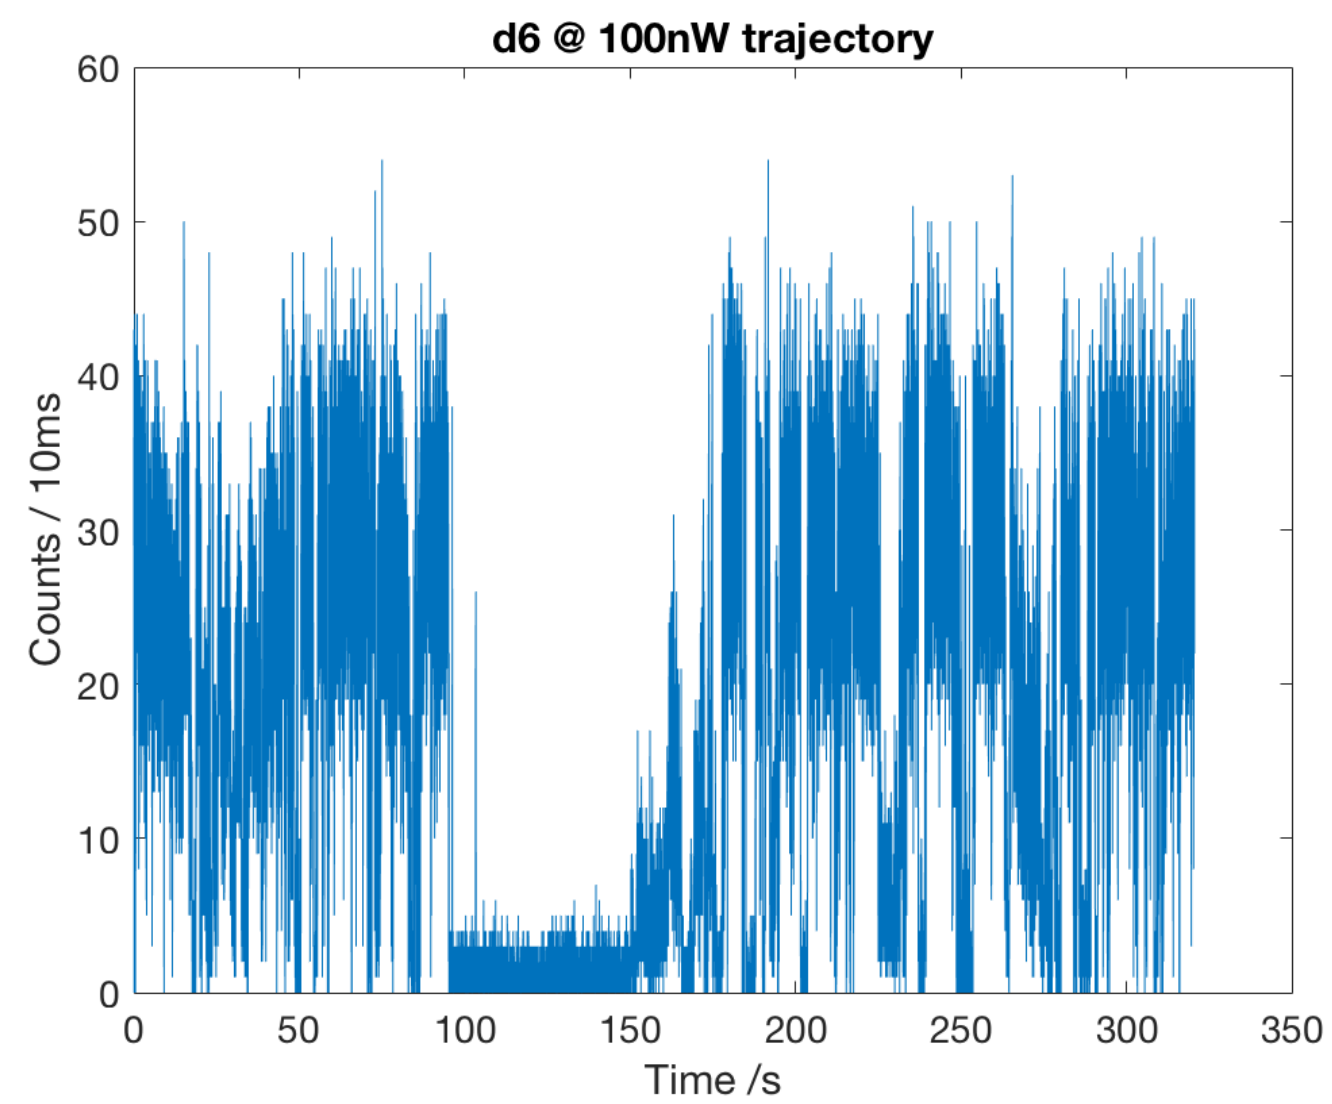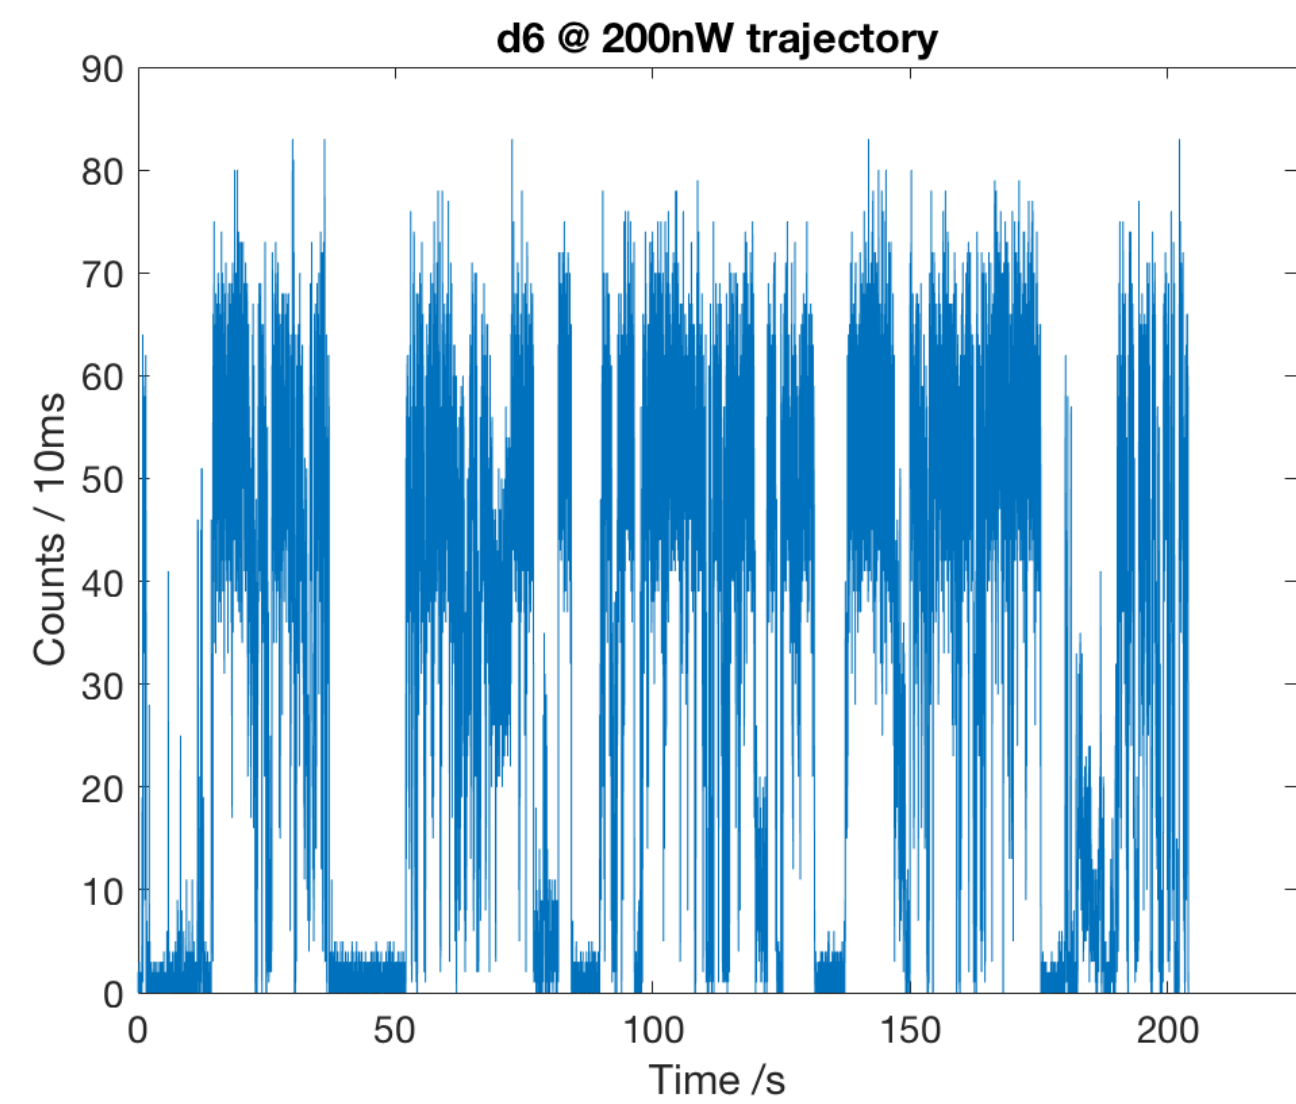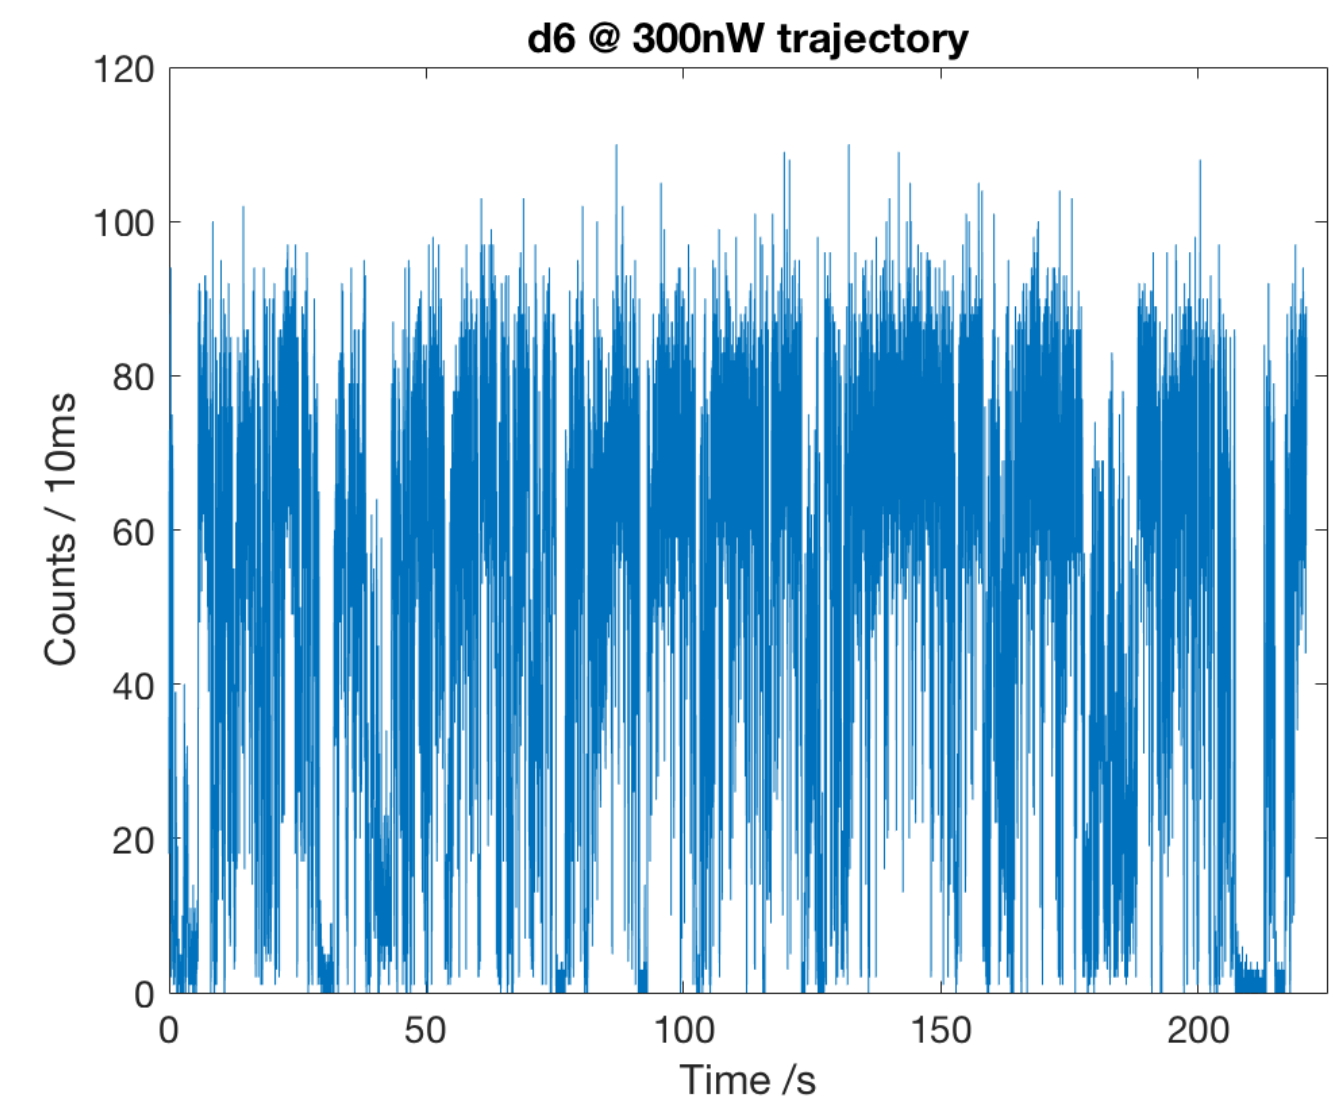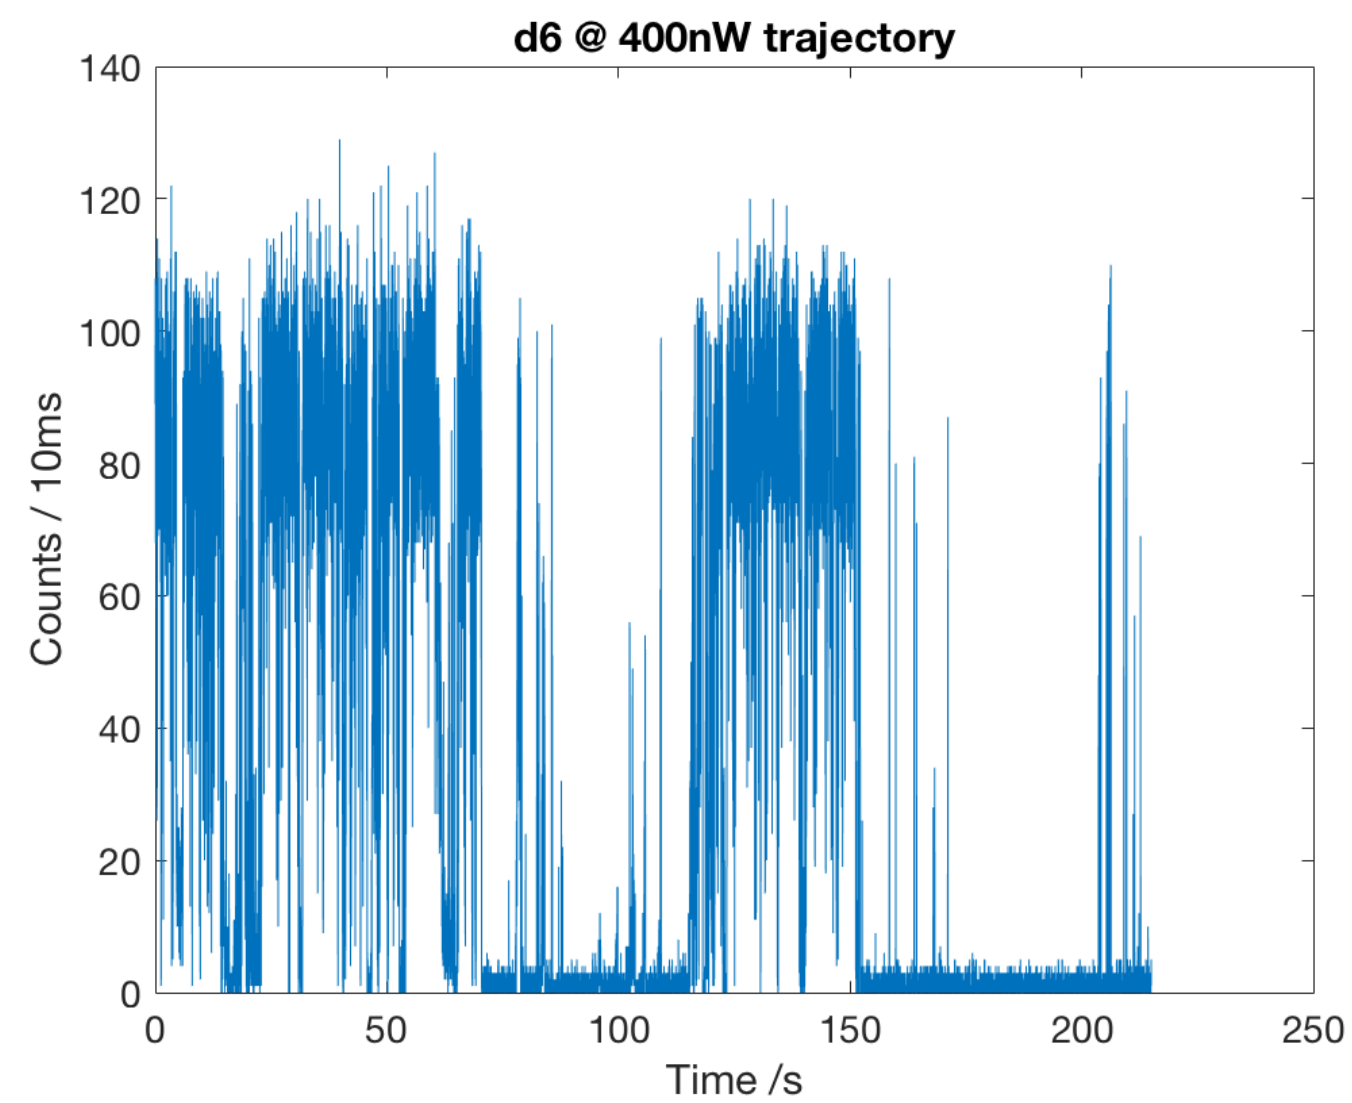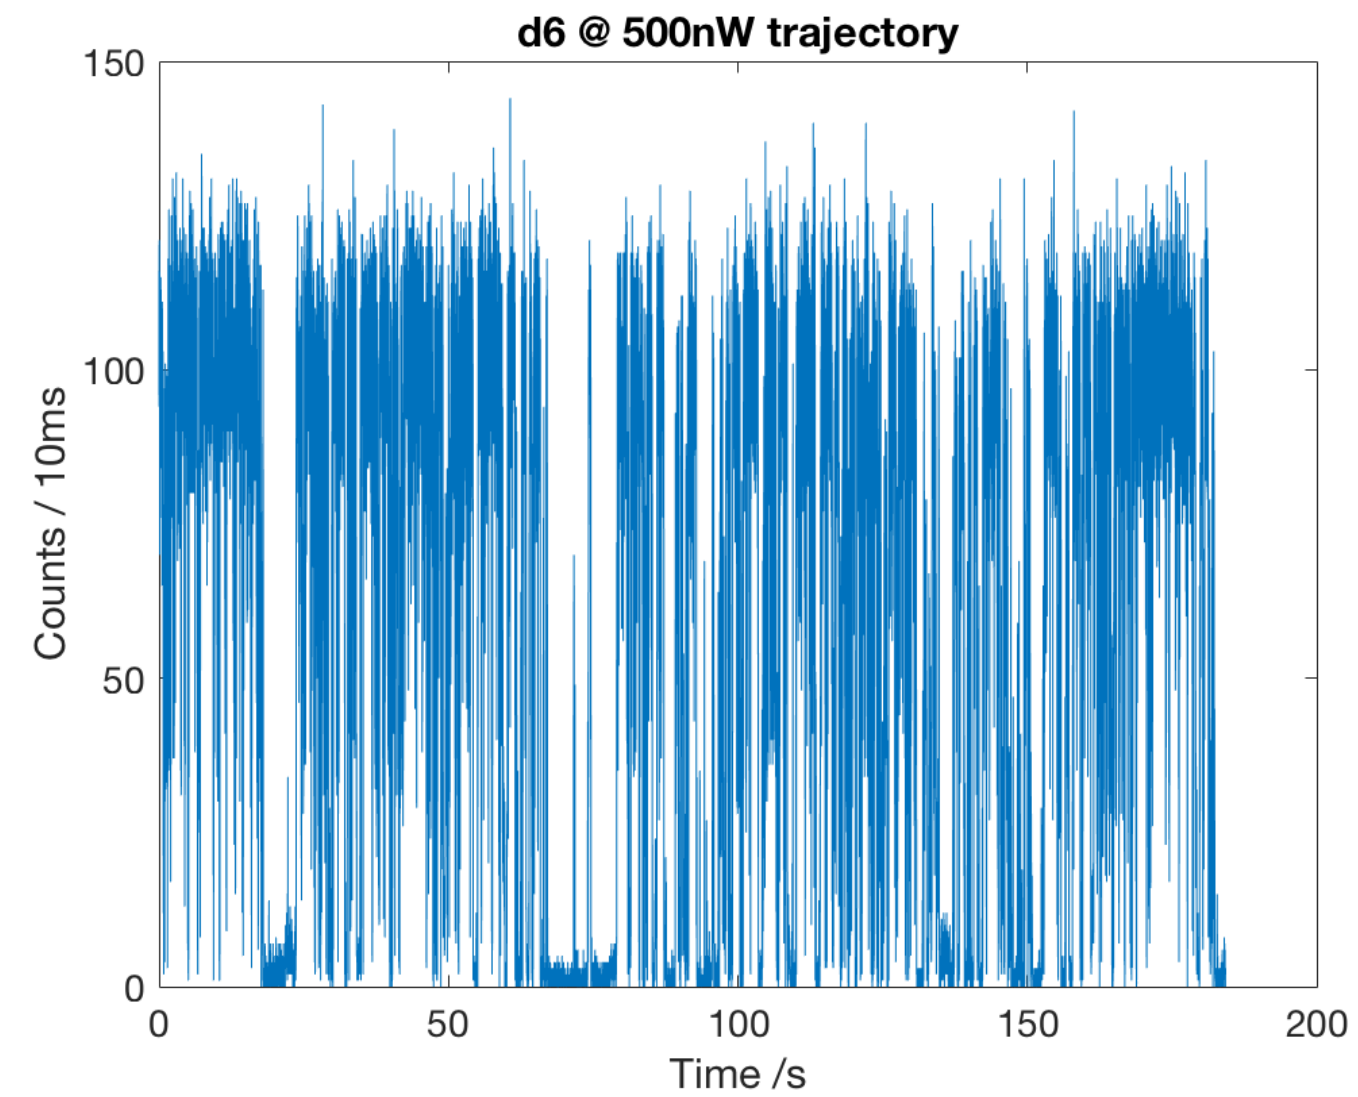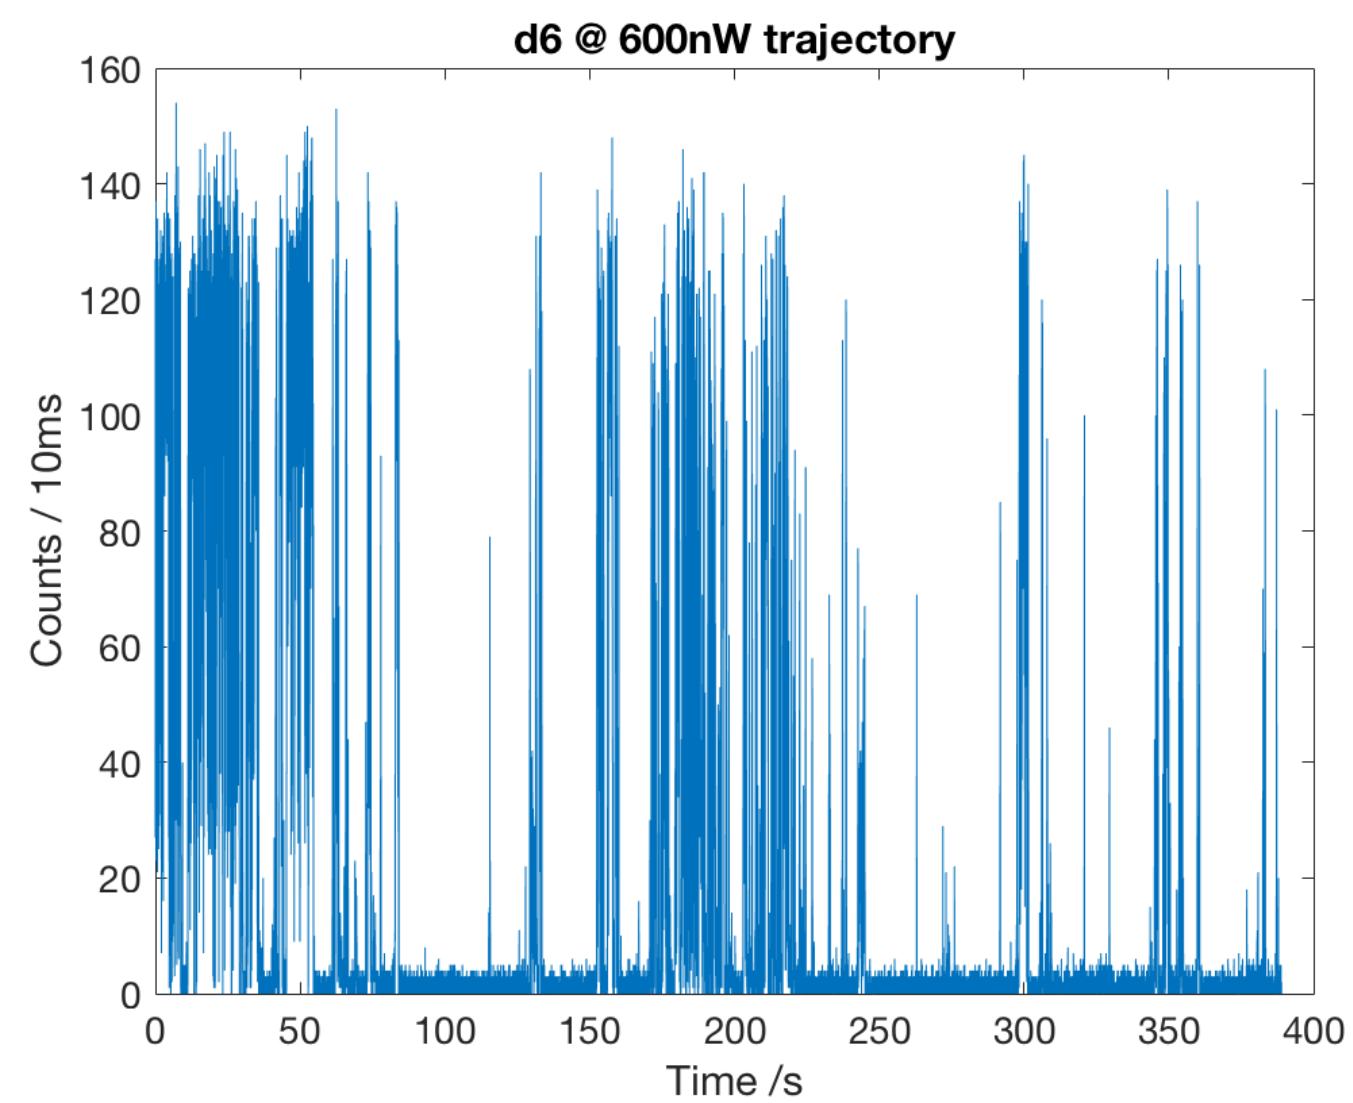

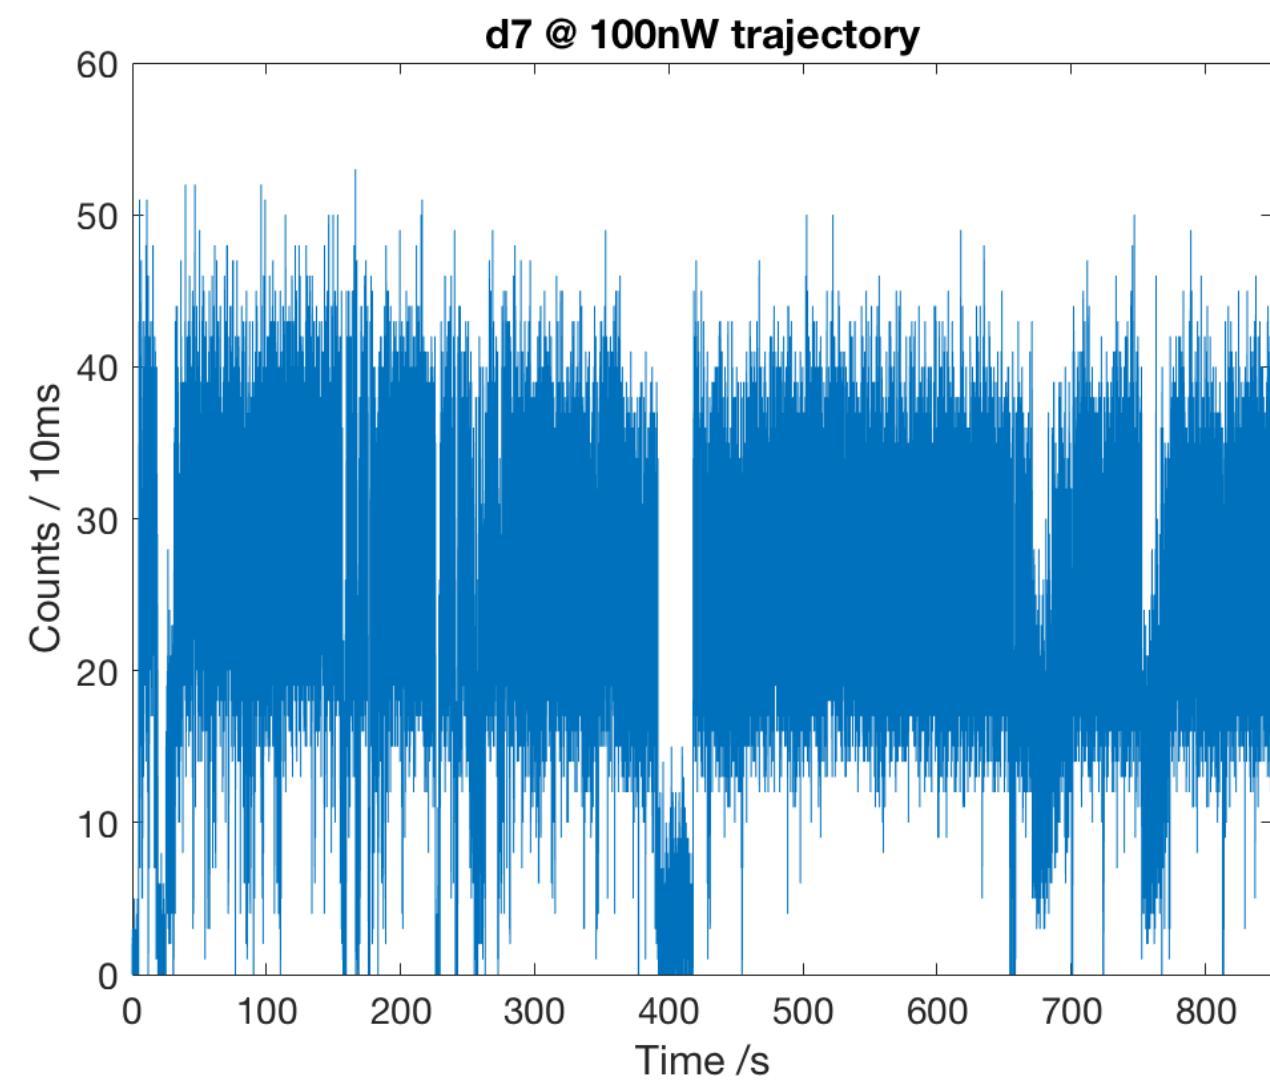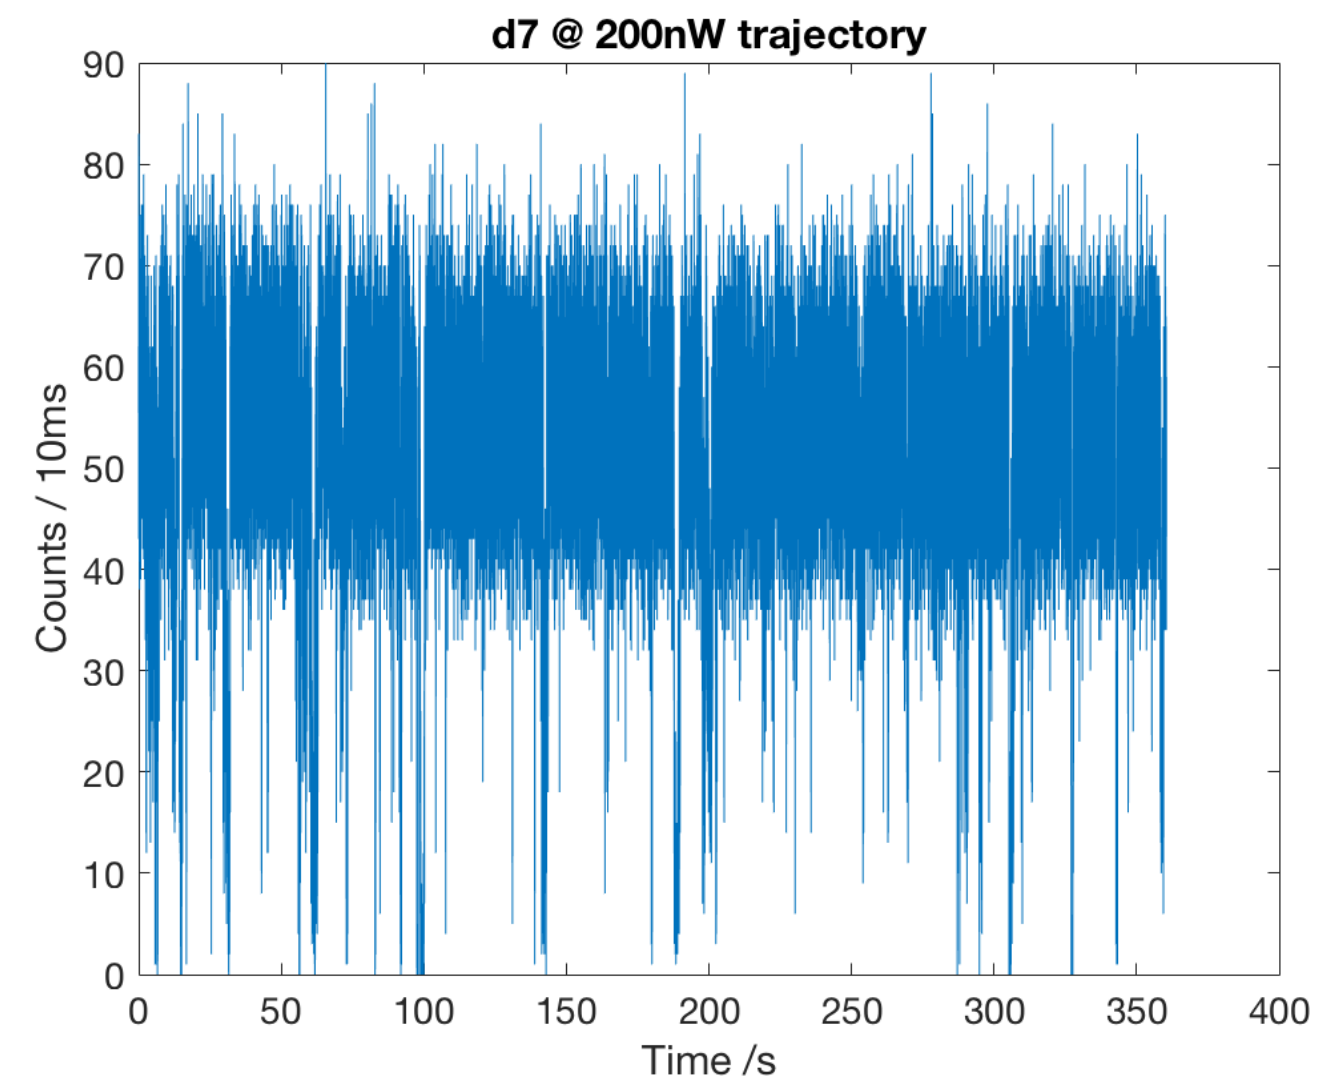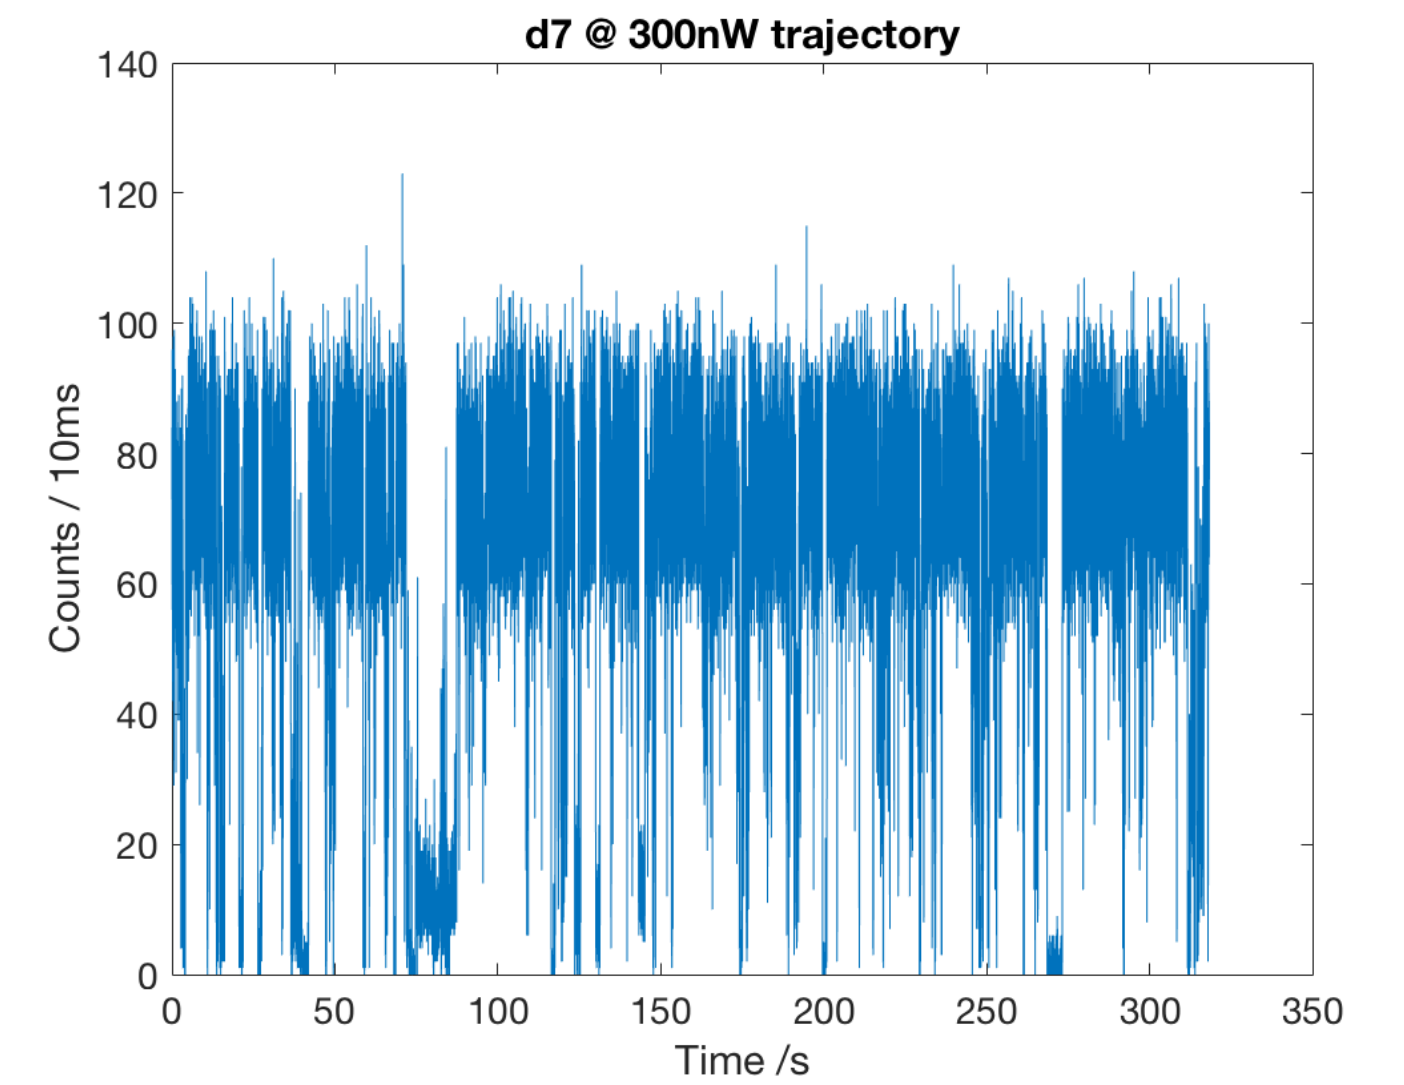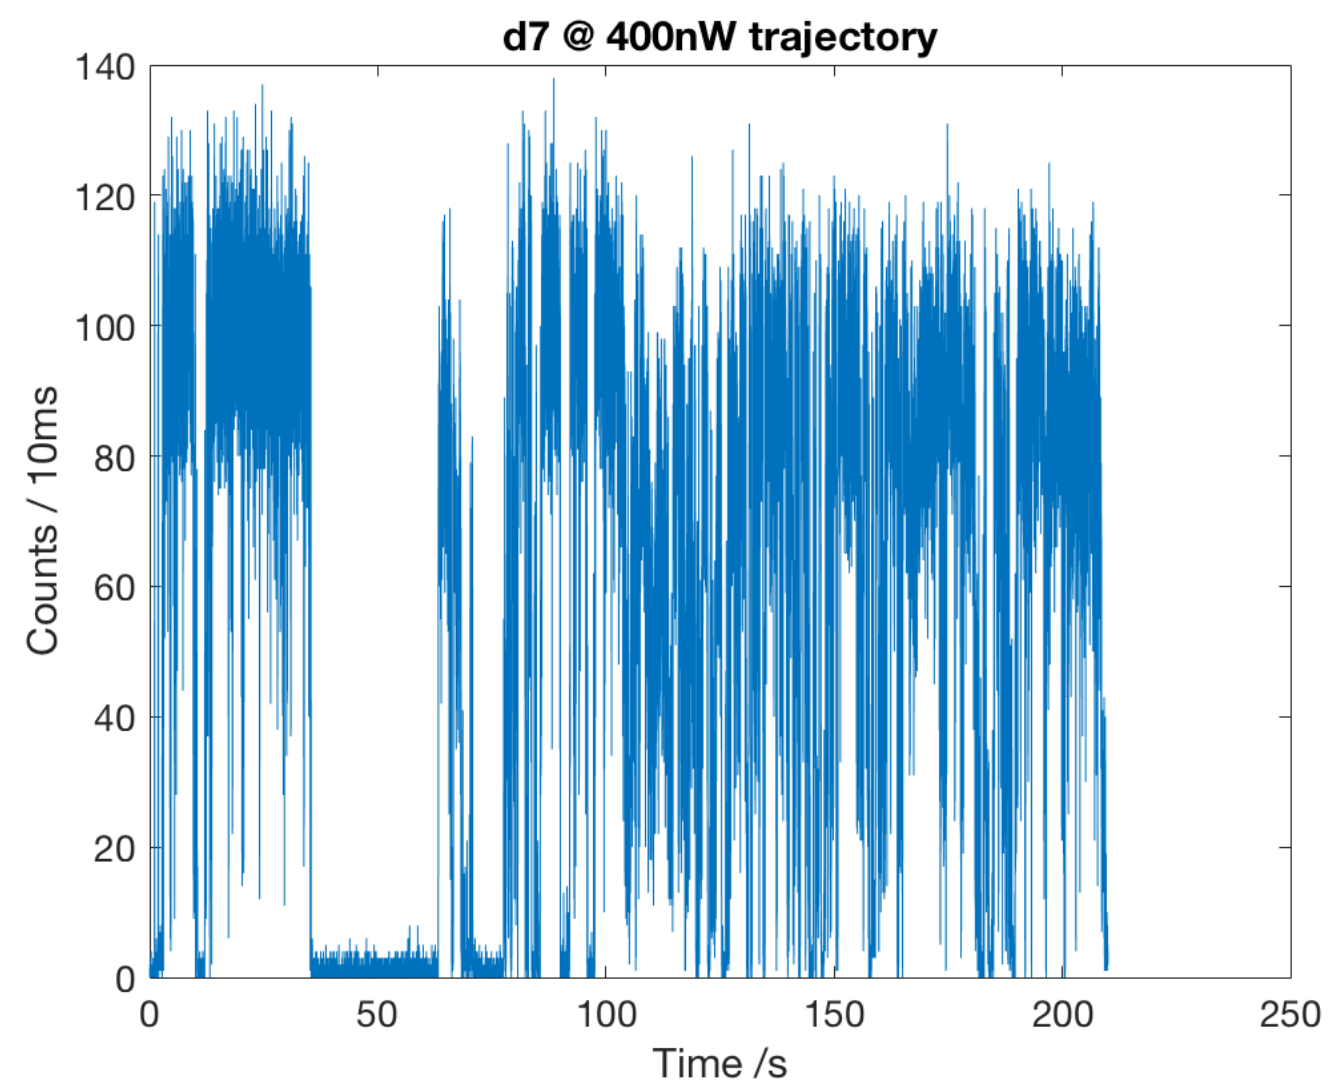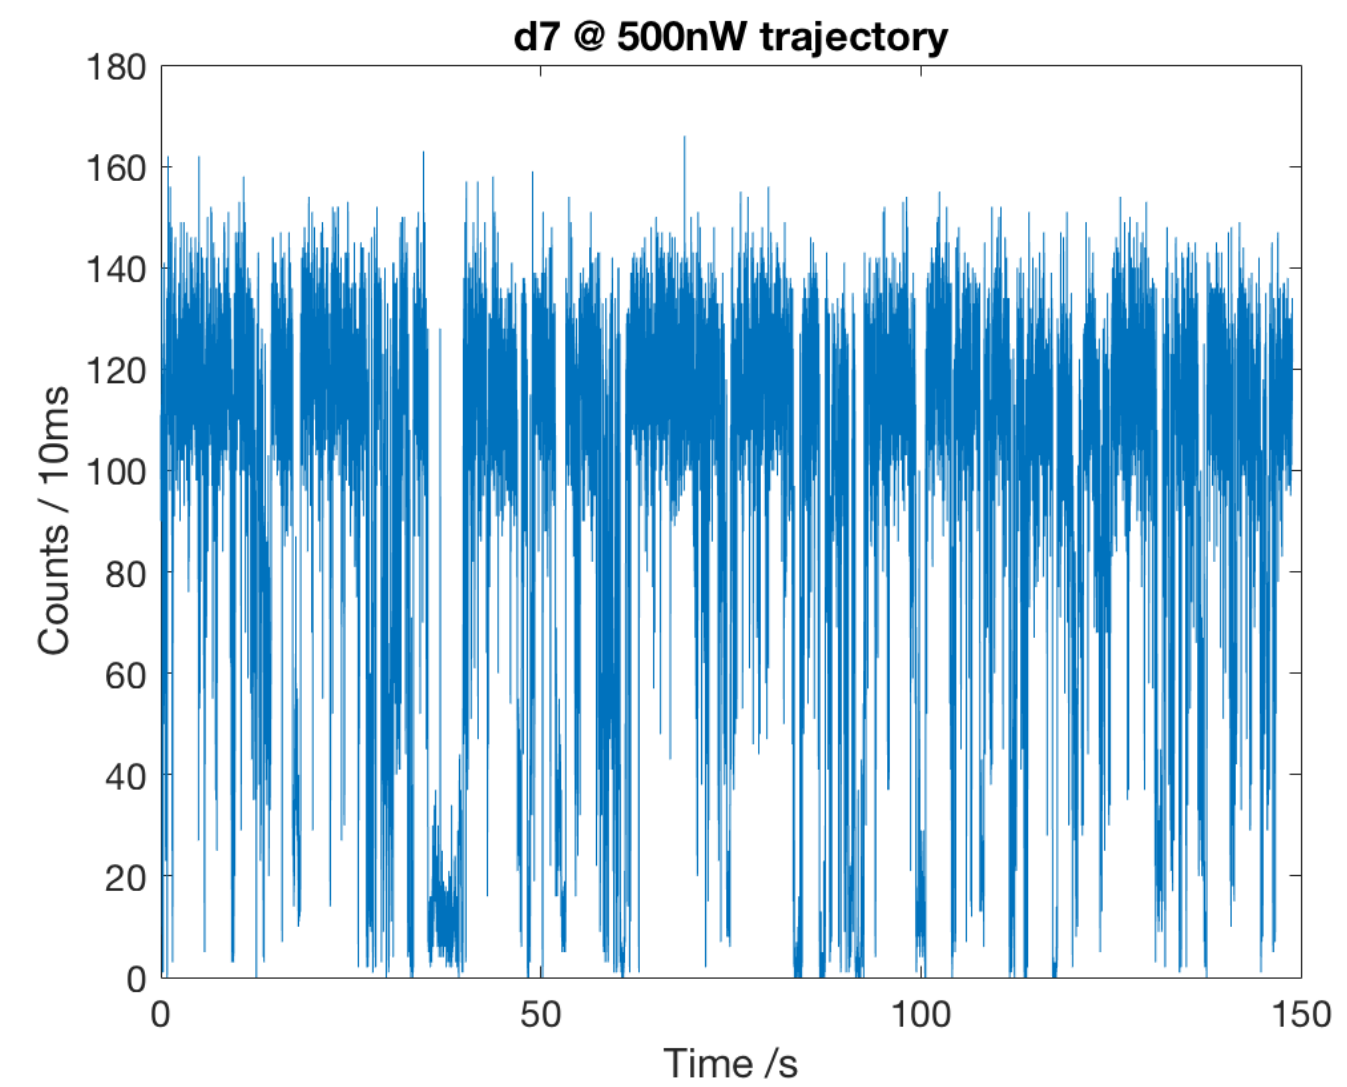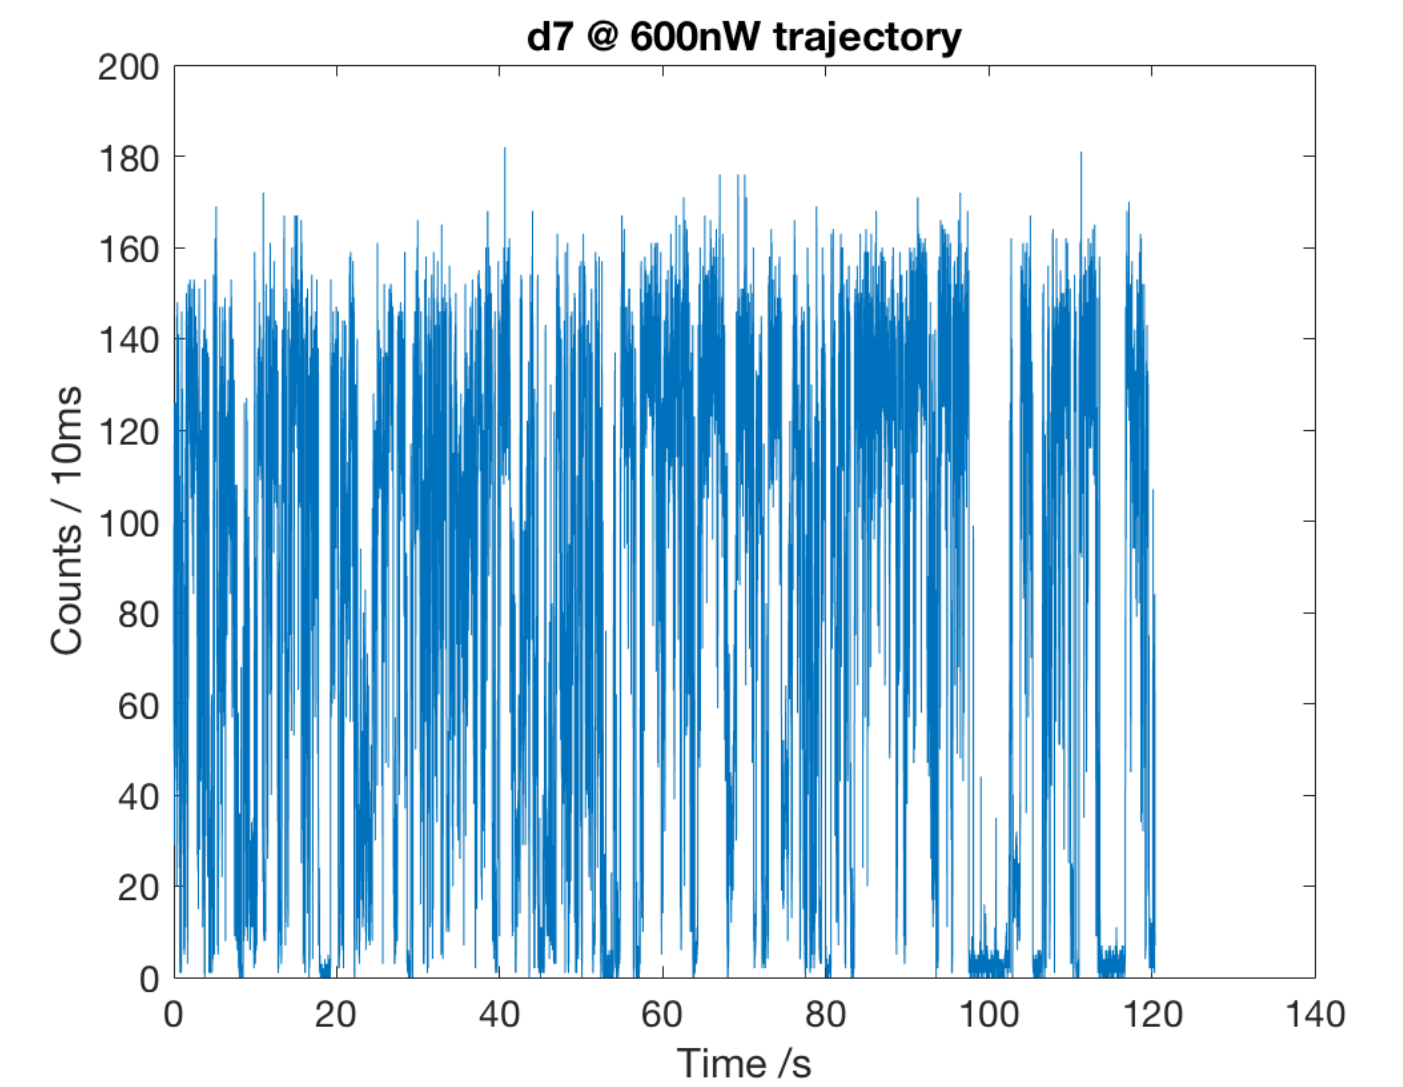

Supplement: Supplementary file 1 [file allDots.pdf]
